# Supplementary material for: MINER: A Hybrid Data-Driven Approach for REST API Fuzzing
Source: arXiv:2303.02545 source file (2023-03-05)
Supplement: Supplementary file 1 [file 10appendix.tex]

\begin{appendix}

   \begin{table*}[b]\scriptsize
    \setlength{\abovecaptionskip}{0.1cm}
\centering
\caption{The proportion of normal, rejection and abnormal responses triggered by RESTler, \sysnamepart and \sysname.} 
\label{table:httpstatuscode}
\begin{tabular}{ccm{1cm}<{\centering}m{1.1cm}<{\centering}m{1.1cm}<{\centering}|m{1.1cm}<{\centering}m{1.1cm}<{\centering}m{1.1cm}<{\centering}|m{1.1cm}<{\centering}m{1.1cm}<{\centering}m{1.1cm}<{\centering}} 
\toprule
\multirow{2}{*}{Cloud Service}    & \multirow{2}{*}{REST API~}  & \multicolumn{3}{c|}{RESTler} & \multicolumn{3}{c|}{\sysnamepart}  & \multicolumn{3}{c}{\sysname}  \\ 
\cline{3-11}
                           &                        & Normal Response       & Rejection Response       & Abnormal Response  & Normal Response       & Rejection Response       & Abnormal Response & Normal Response       & Rejection Response       & Abnormal Response      \\ 
\toprule
\multirow{5}{*}{GitLab}    & Projects               & 71.86\%   & 27.99\%   &0.15\%  &  95.50\% & 4.23\% & 0.27\%   & 95.52\%& 4.22\%& 0.26\%   \\
                           & Groups                 & 64.12\%  & 34.99\%   &0.89\%&  90.58\% & 7.63\%&1.79\%     & 89.82\%& 7.72\%& 2.46\%         \\
                           & Issues                 & 86.55\%   & 13.44\%   &7.82e$^{-4}$& 96.02\%  &3.87\%  & 0.11\%  & 95.29\%& 4.58\%& 0.13\%            \\ 
                           & Commits                 & 53.26\%   & 46.48\%   &0.26\%      & 86.46\%  & 13.35\% & 0.19\%  & 86.21\% & 13.30\% &0.49\%     \\
                           & Branches               & {81.07\%}   & {18.90\%}     & {3.59e$^{-4}$} & {89.86\%}  & {10.09\%} & {5.39$^{-4}$} &   {89.21\%} & {10.69\%} &{0.10\%}                                                                                           \\
\hline
\multirow{3}{*}{Bugzilla}  & Comments               & 87.93\%   &  11.21\%  & 0.86\% &  89.57\% &  10.26\%& 0.17\% & 89.87\% &  9.77\%  & 0.36\%         \\
& Bugs                   & 37.64\%   & 54.07\%     & 8.29\% &  88.65\% &  8.95\% & 2.40\% & 89.43\% &  6.84\%  & 3.73\%      \\
                           & Groups                 & 54.26\%   & 45.12\%   & 0.62\% &  73.30\% & 25.99\% & 0.71\% & 72.16\%&  27.15\%  & 0.69\% \\
\hline
% \multirow{3}{*}{Jira}      & Projects               &            &          &      &            &          &     &            &          &          \\
%                           & Issues                 &            &          &      &            &          &     &            &          &          \\
%                           & Worklogs                &            &          &      &            &          &     &            &          &          \\ 
% \hline
\multirow{3}{*}{WordPress} & Categories             & 61.38\%    & 24.67\%  &13.95\%&  90.45\%  & 8.04\% &  1.51\%   &  90.08\% & 7.36\%   &2.56\%          \\
& Posts                  & 94.05\%    &  5.94\%  &6.32e$^{-5}$&  95.12\%  & 4.87\% &7.32e$^{-5}$  &    95.56\% &   4.44\% & 6.65e$^{-5}$        \\
                           & Comments               & 96.61\%    &  3.39\%  &  0.00\%    &  99.65\%  & 0.35\% &  0.00\%     &   99.43\%  &   0.57\%  &   0.00\%       \\
\toprule
\end{tabular}
\end{table*}

\section{Proportion of Request Responses}\label{sec:qualityanalysis}

To  analyze the generation quality of requests, 
we further measure the proportion of different responses 
triggered by each fuzzer based on the results in Section~\ref{sec:fuzzingperformance}. 
 The results are shown in Table~\ref{table:httpstatuscode}, 
and we have the following conclusion. 
%\textbf{Our design can significantly increase the proportion of the normal responses.}  %the responses in \texttt{20$\times$} Range.} 
{Our approach significantly improves the generation quality of requests, 
which significantly reduces the number of rejection responses  
and increases the proportion of the normal responses.} 
For instance, the proportion of the normal responses 
triggered by \sysnamepart is 32.90\% higher than RESTler on GitLab Projects API, 
and the proportion of the normal responses 
triggered by \sysnamepart is 62.34\% higher than RESTler on GitLab Commits API. 
These results demonstrate the contribution of our approach to request generation. 
Note that \sysnamepart can benefit from generating valid requests and getting normal responses. 
For instance, by generating valid {consumers} and getting normal responses, 
\sysnamepart  successfully provides target object ids for {producers}, 
which improves the complexity of request sequences.  

On the other hand, we can see that the proportion of the abnormal responses 
is smaller than 4.00\% in 31 of all the 33 results, which implies that the requests triggering abnormal responses %the responses in \texttt{50$\times$} Range  
are pretty rare in the fuzzing process. 
Thus, these data are insufficient to train a meaningful machine learning model in our application scenario.
Nevertheless,  for different application scenarios like continuous fuzzing, which may have plenty of previous fuzzing data, 
\sysnamepart can utilize another attention model to 
generate the \textit{parameter combinations} 
that can trigger abnormal responses. %the response of \texttt{50$\times$} Range. 

\section{Sequence Length Analysis}\label{sec:sequencelengthanalysis}

To analyze the contribution of different designs to sequence length, 
we conduct the experiments as follows. 
We evaluate RESTler, RESTler+Seq, RESTler+Model, and \sysnamepart on GitLab Projects API, GitLab Groups API, GitLab Issues API, Bugzilla Comments API, and WordPress Categories API. 
Each evaluation lasts for 12 hours, during which we count the executions of sequences with different lengths. 
Based on the above settings, 
we can measure the contribution of the \emph{attention model-based request generation} to sequence length from the results of RESTler and RESTler+Model, and the results of RESTler+Seq and \sysnamepart. 
We can measure the contribution of the \emph{length orientated sequence construction} to sequence length from the results of RESTler and RESTler+Seq, and the results of RESTler+Model and \sysnamepart. 
Since the \emph{DataDriven Checker} does not affect the sequence extension, 
%we do not measure the performance of \sysnameplus. 
we omit \sysname in the evaluation. 
%we do not include \sysnameplus in the evaluation. 
The results are shown in Fig.~\ref{fig:seqlength}, from which we have the following conclusions.

\begin{figure*}[t]
 \setlength{\abovecaptionskip}{0.2cm}
 \setlength{\belowcaptionskip}{-0.01cm}
     \centering
     \begin{subfigure}[b]{0.33\textwidth}    
         \centering
         \includegraphics[width=2.3in,height=1.9in]{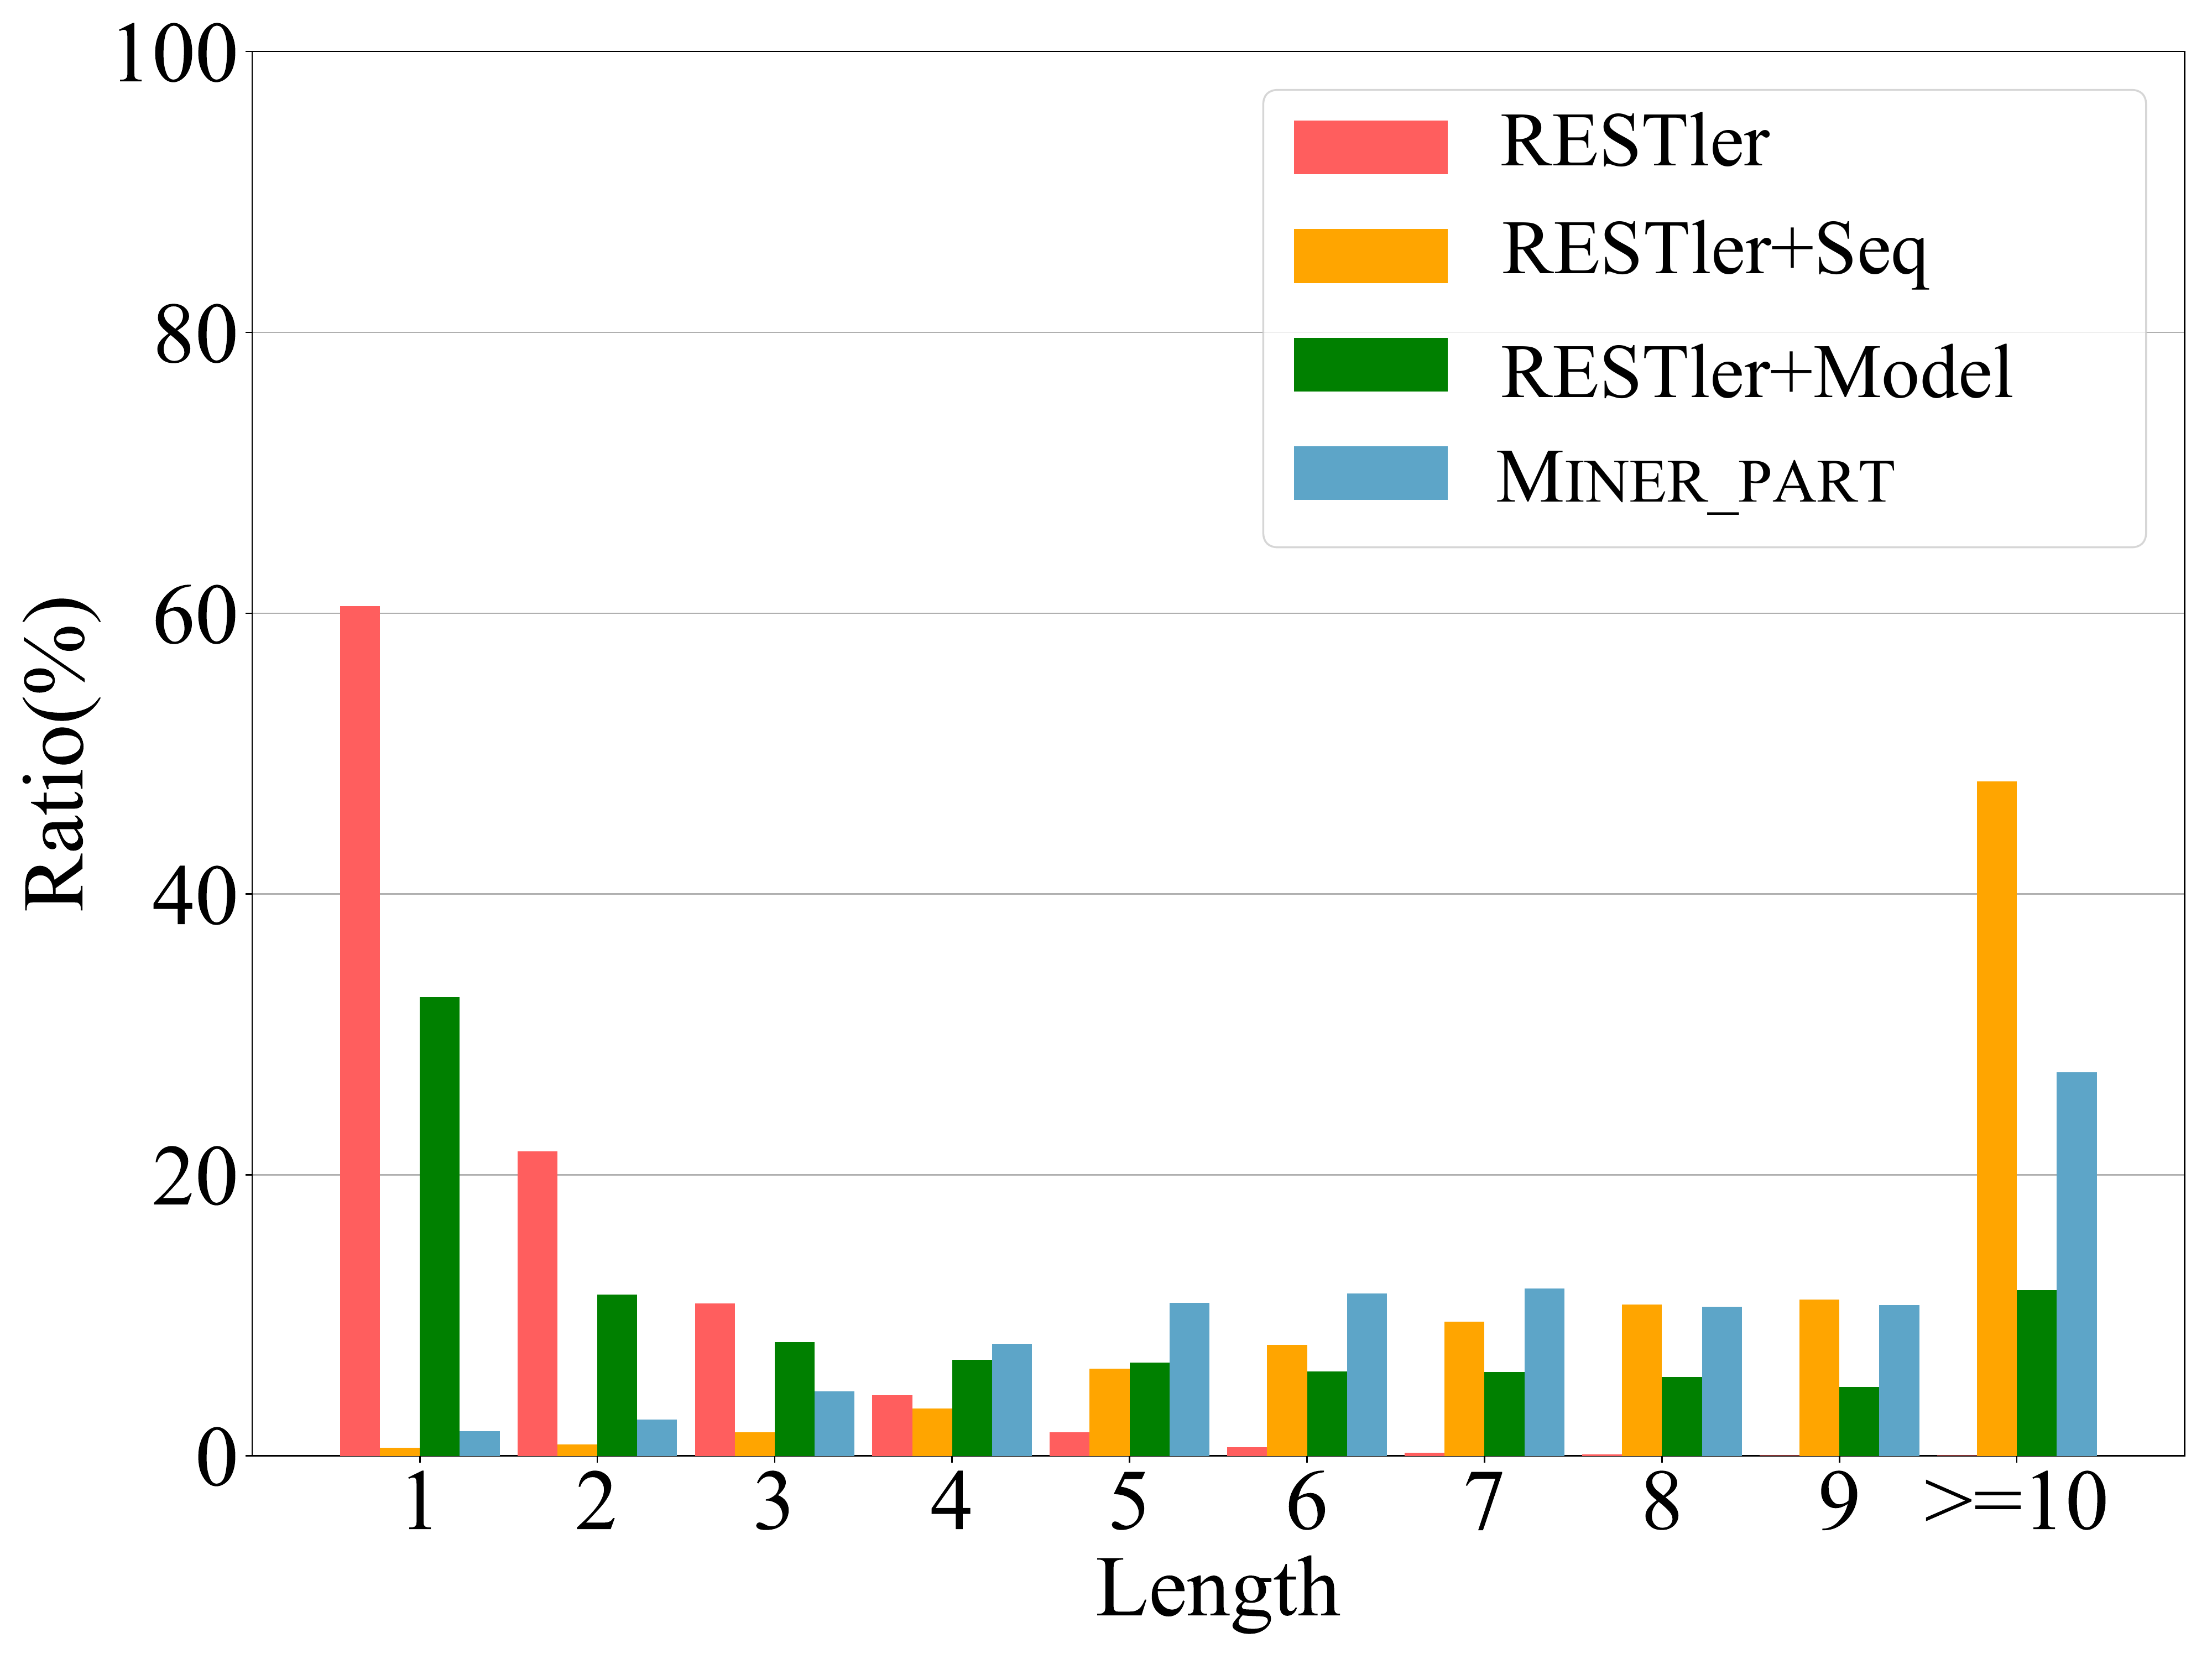}
          \setlength{\abovecaptionskip}{-0.4cm}
         \caption{GitLab Projects API.}
         %\label{fig:y equals x}
     \end{subfigure}
     \hfill
     \begin{subfigure}[b]{0.33\textwidth}    
         \centering
         \includegraphics[width=2.3in,height=1.9in]{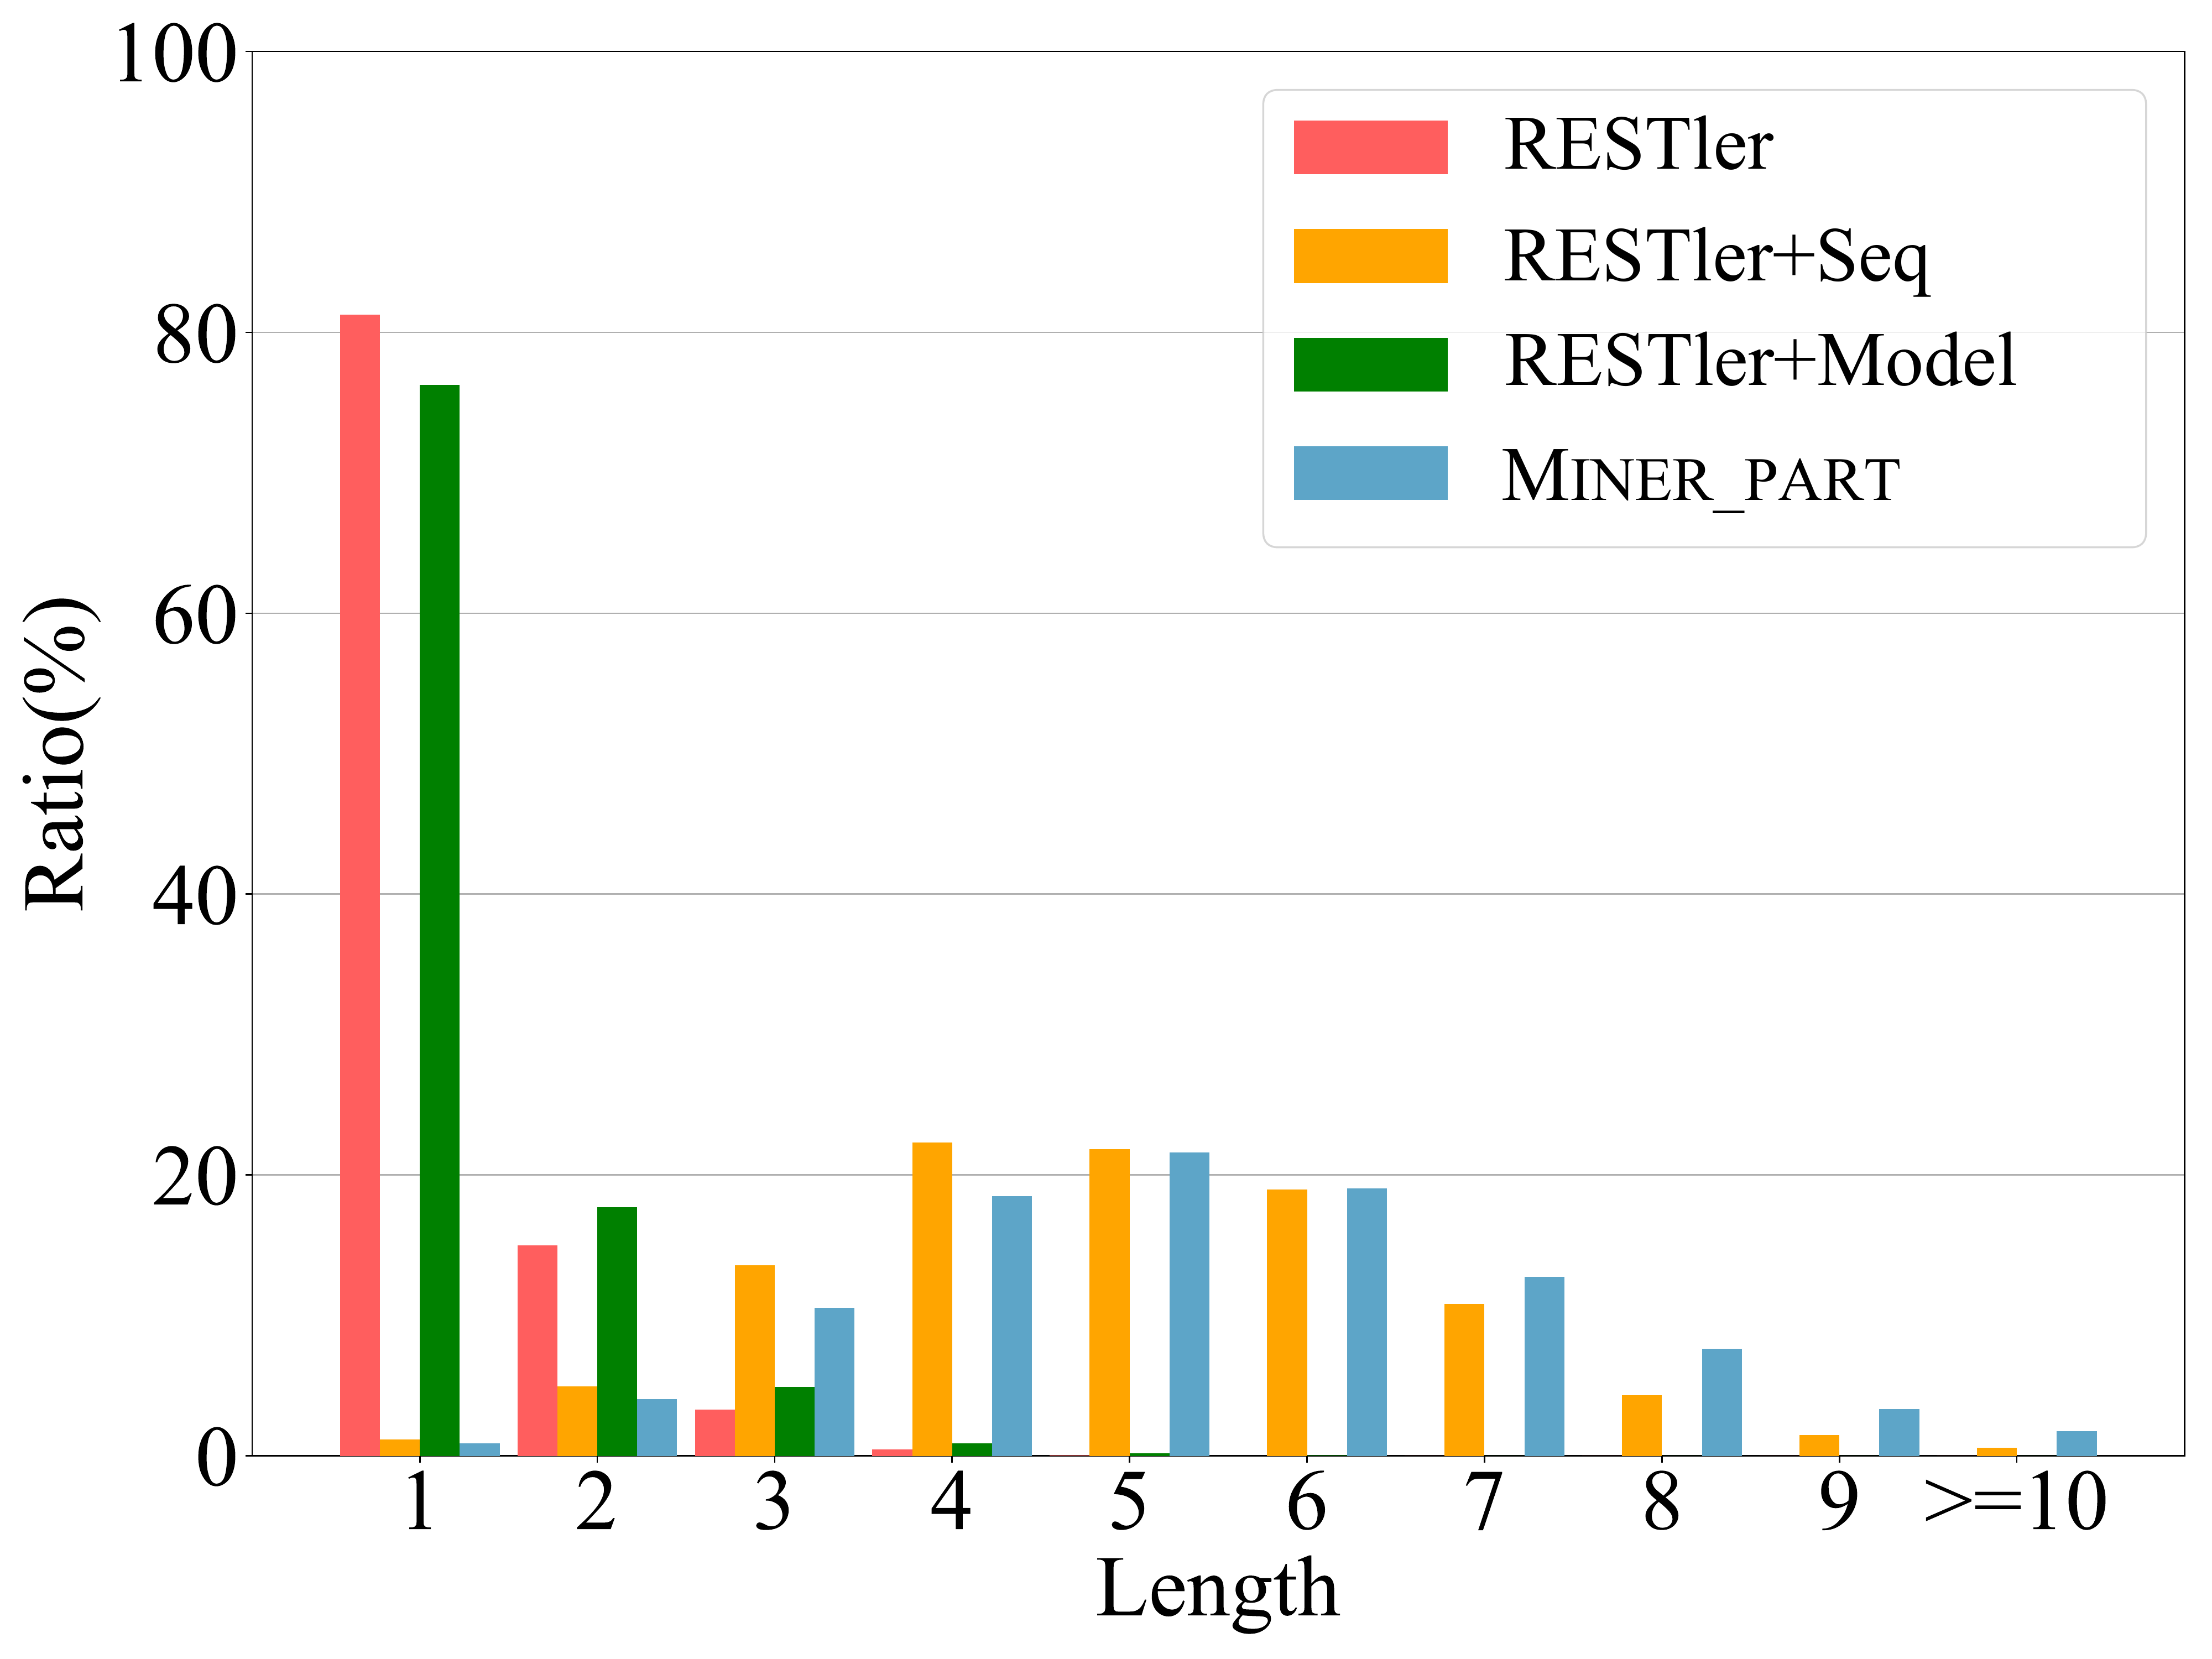}
         \setlength{\abovecaptionskip}{-0.4cm}
         \caption{GitLab Groups API.}
         %\label{fig:three sin x}
     \end{subfigure}
     \hfill
     \begin{subfigure}[b]{0.33\textwidth}    
         \centering
         \includegraphics[width=2.3in,height=1.9in]{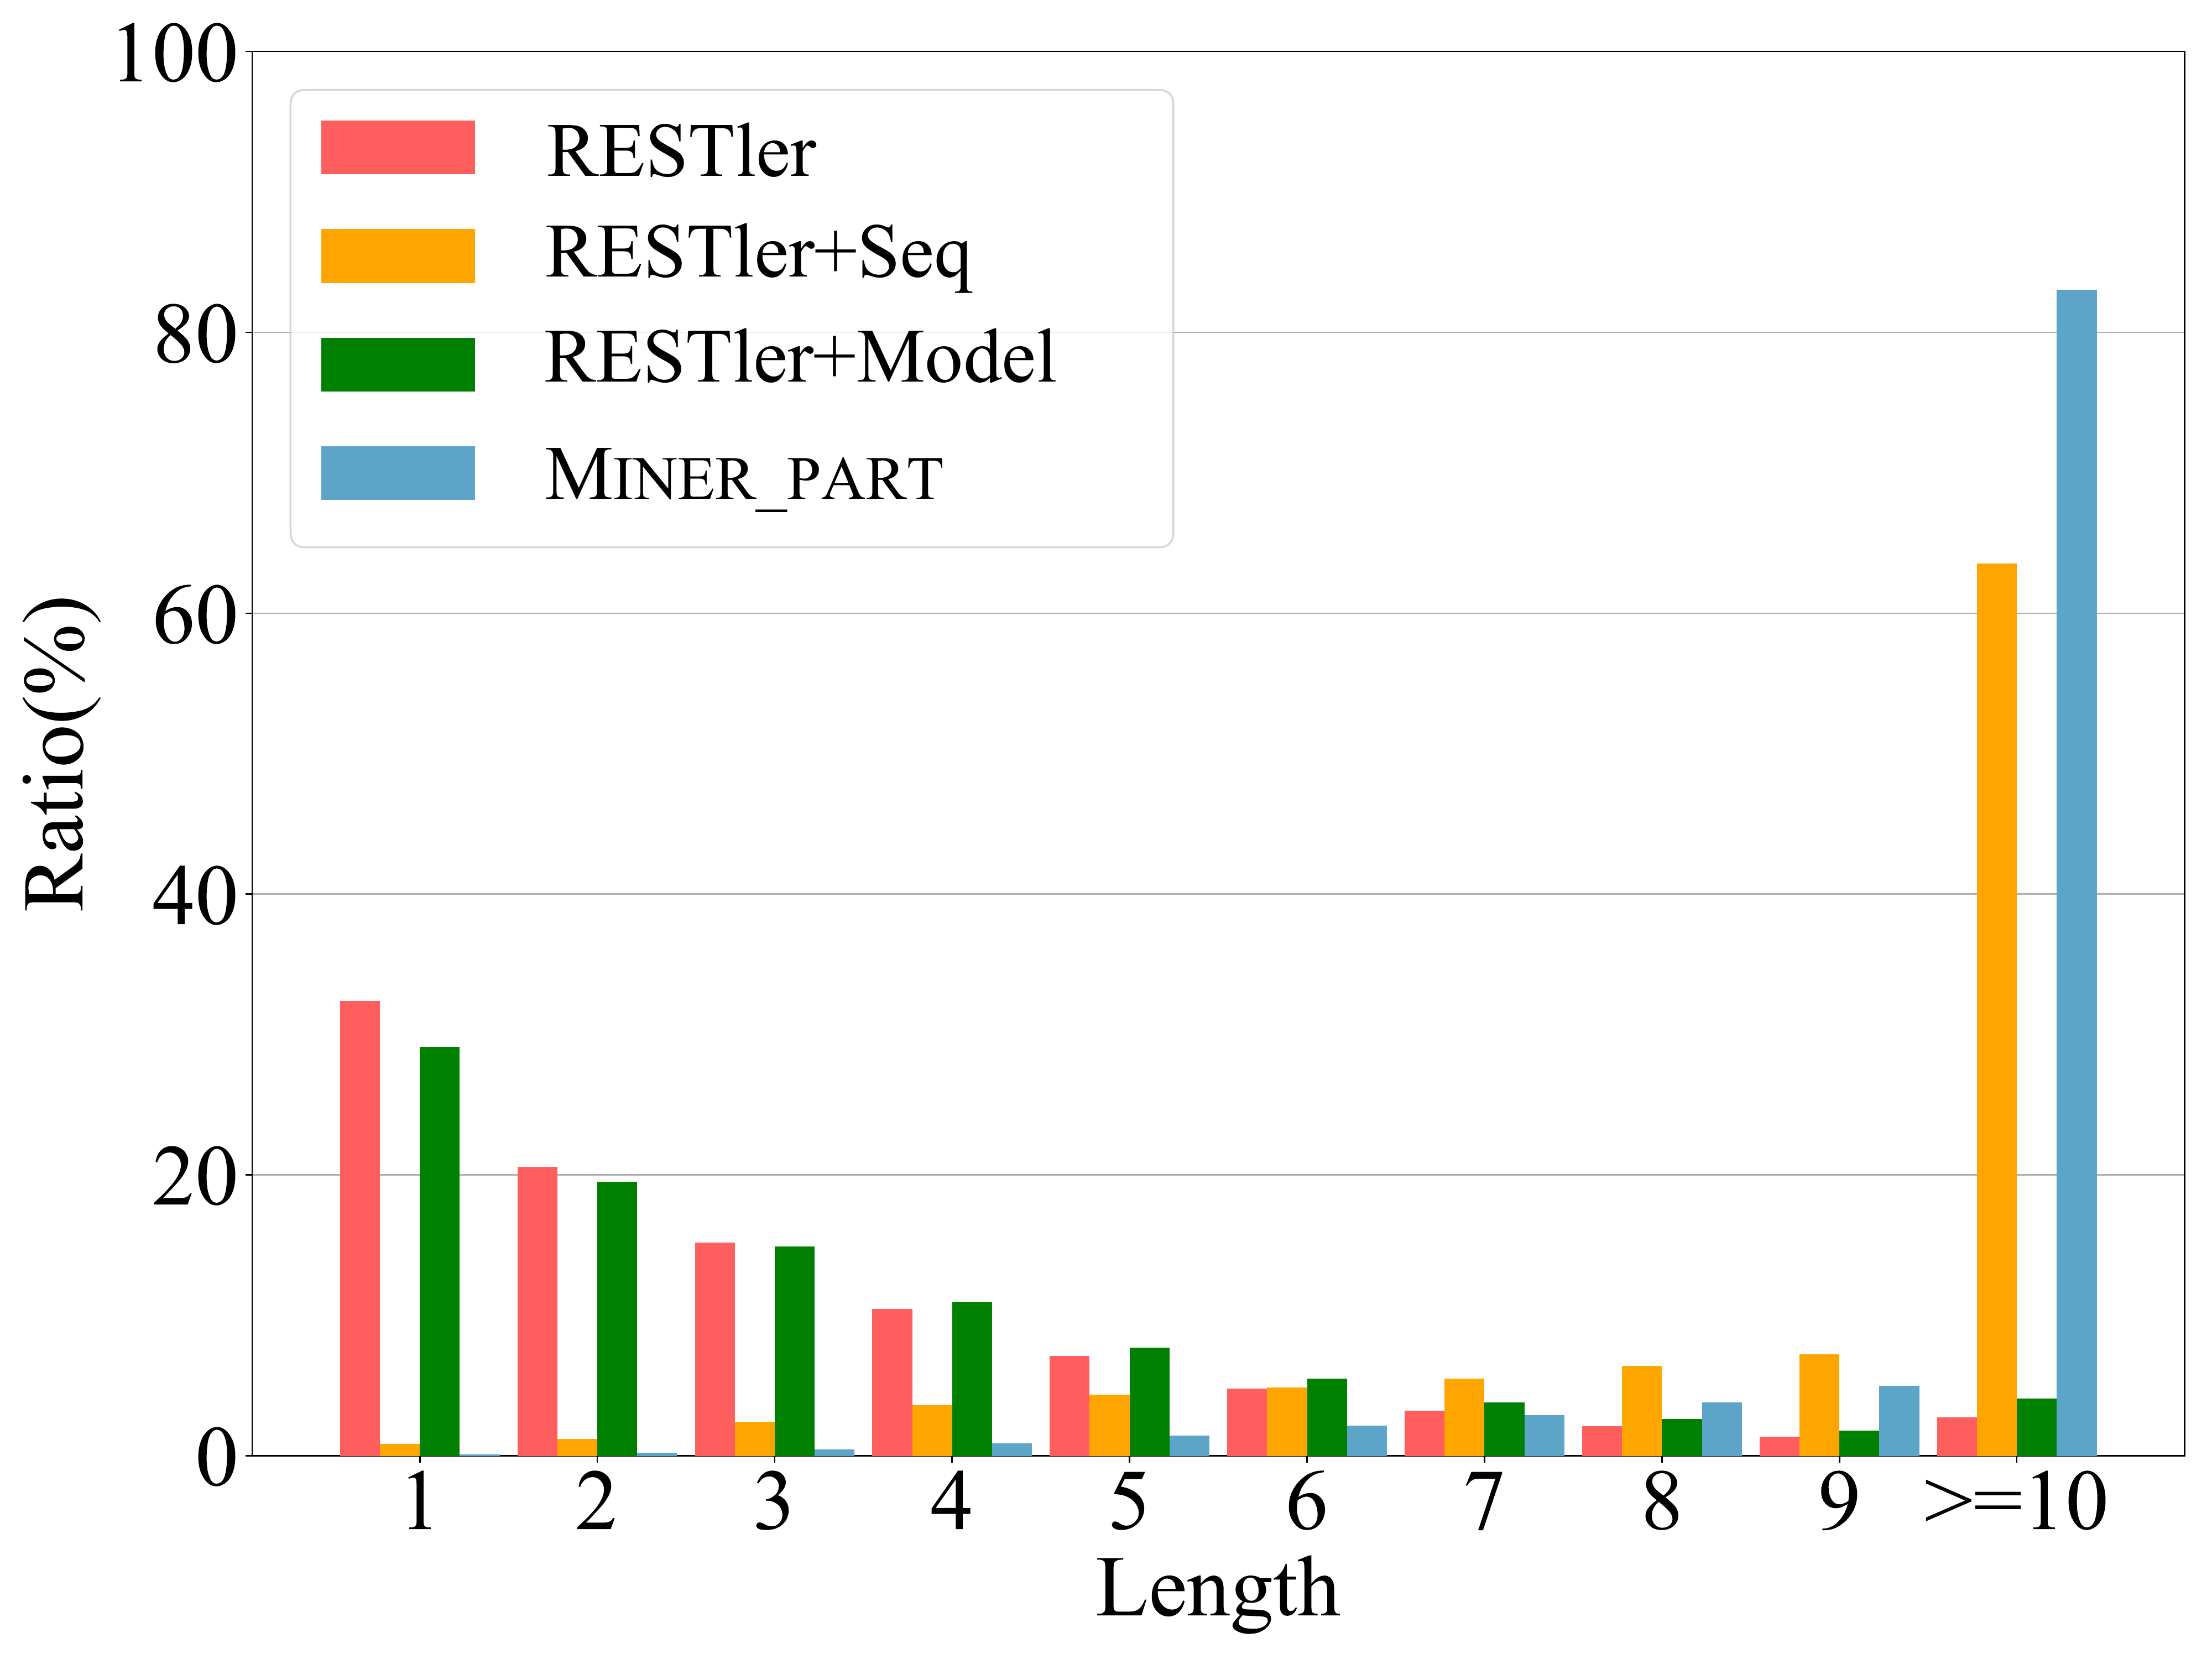}
         \setlength{\abovecaptionskip}{-0.4cm}
         \caption{GitLab Issues API.}
         %\label{fig:five over x}
     \end{subfigure}
     \hfill
\hspace{1mm}
     \begin{minipage}[!htb]{1\linewidth}
     \centering
        \begin{subfigure}[b]{0.33\textwidth}
            \centering
            \includegraphics[width=2.3in,height=1.9in]{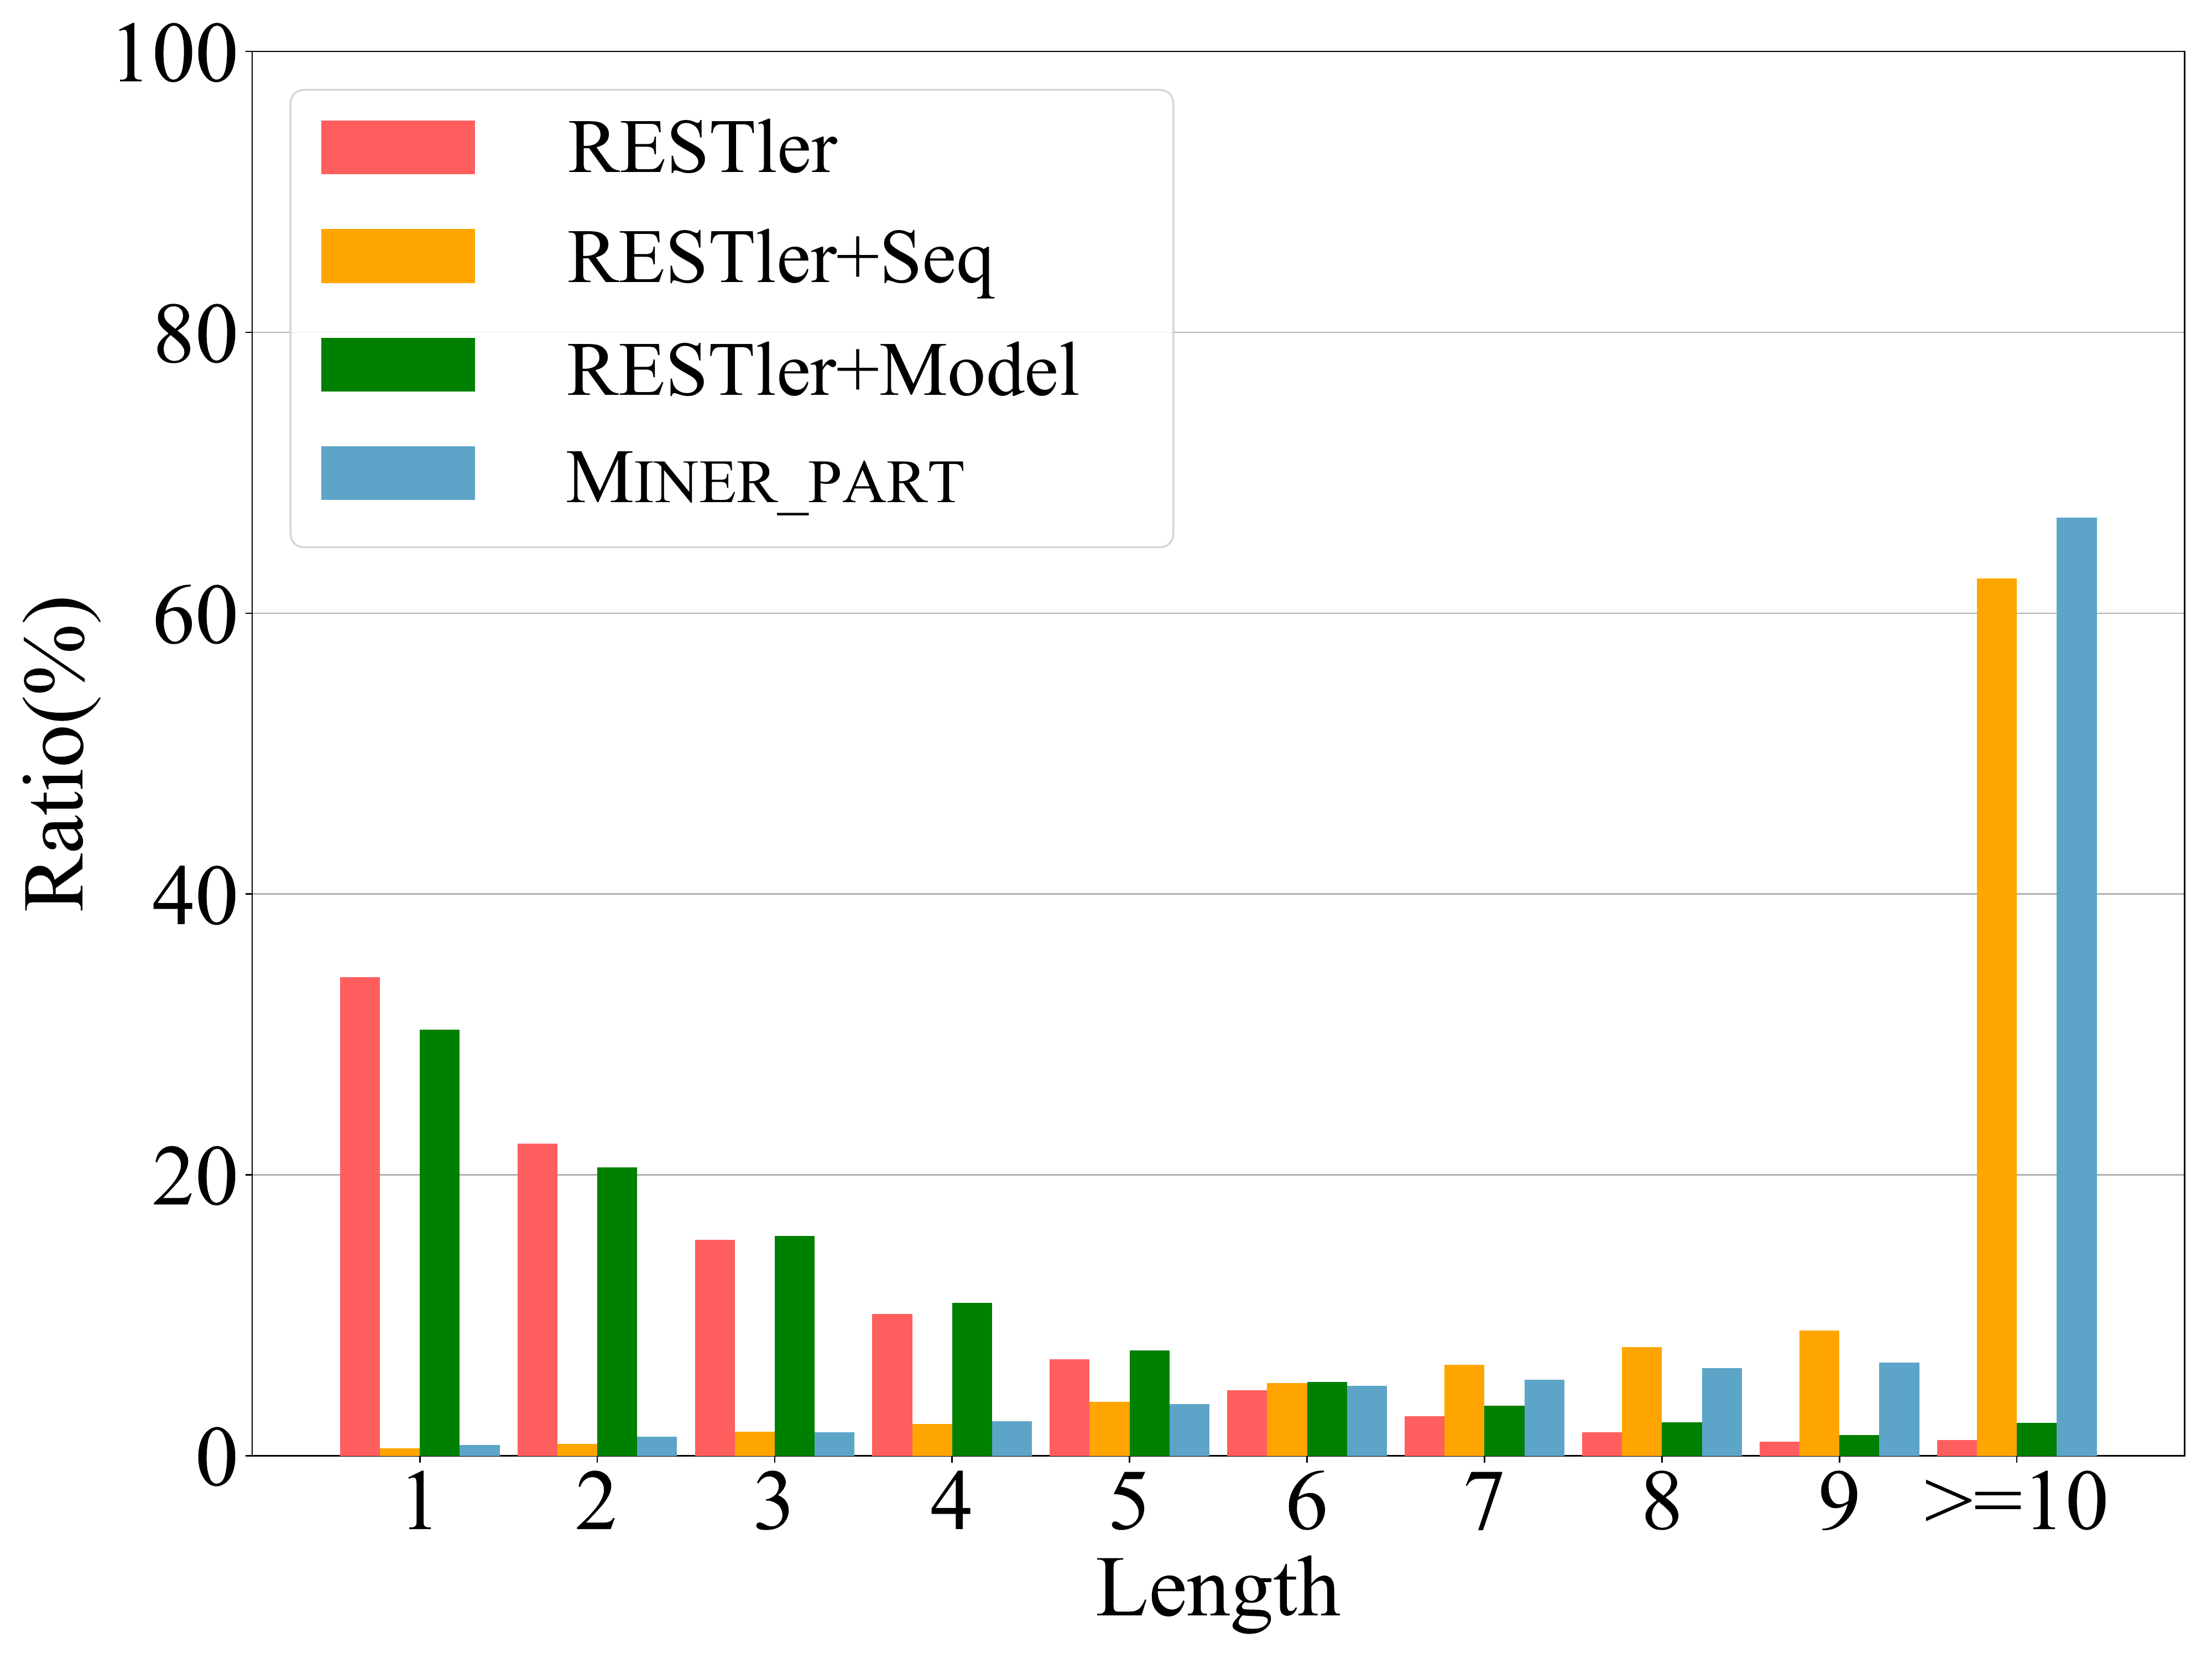}
            \setlength{\abovecaptionskip}{-0.4cm}
            \caption{Bugzilla Comments API.}
            %\label{fig:five over x}
        \end{subfigure}
        \begin{subfigure}[b]{0.33\textwidth}
            \centering
            \includegraphics[width=2.3in,height=1.9in]{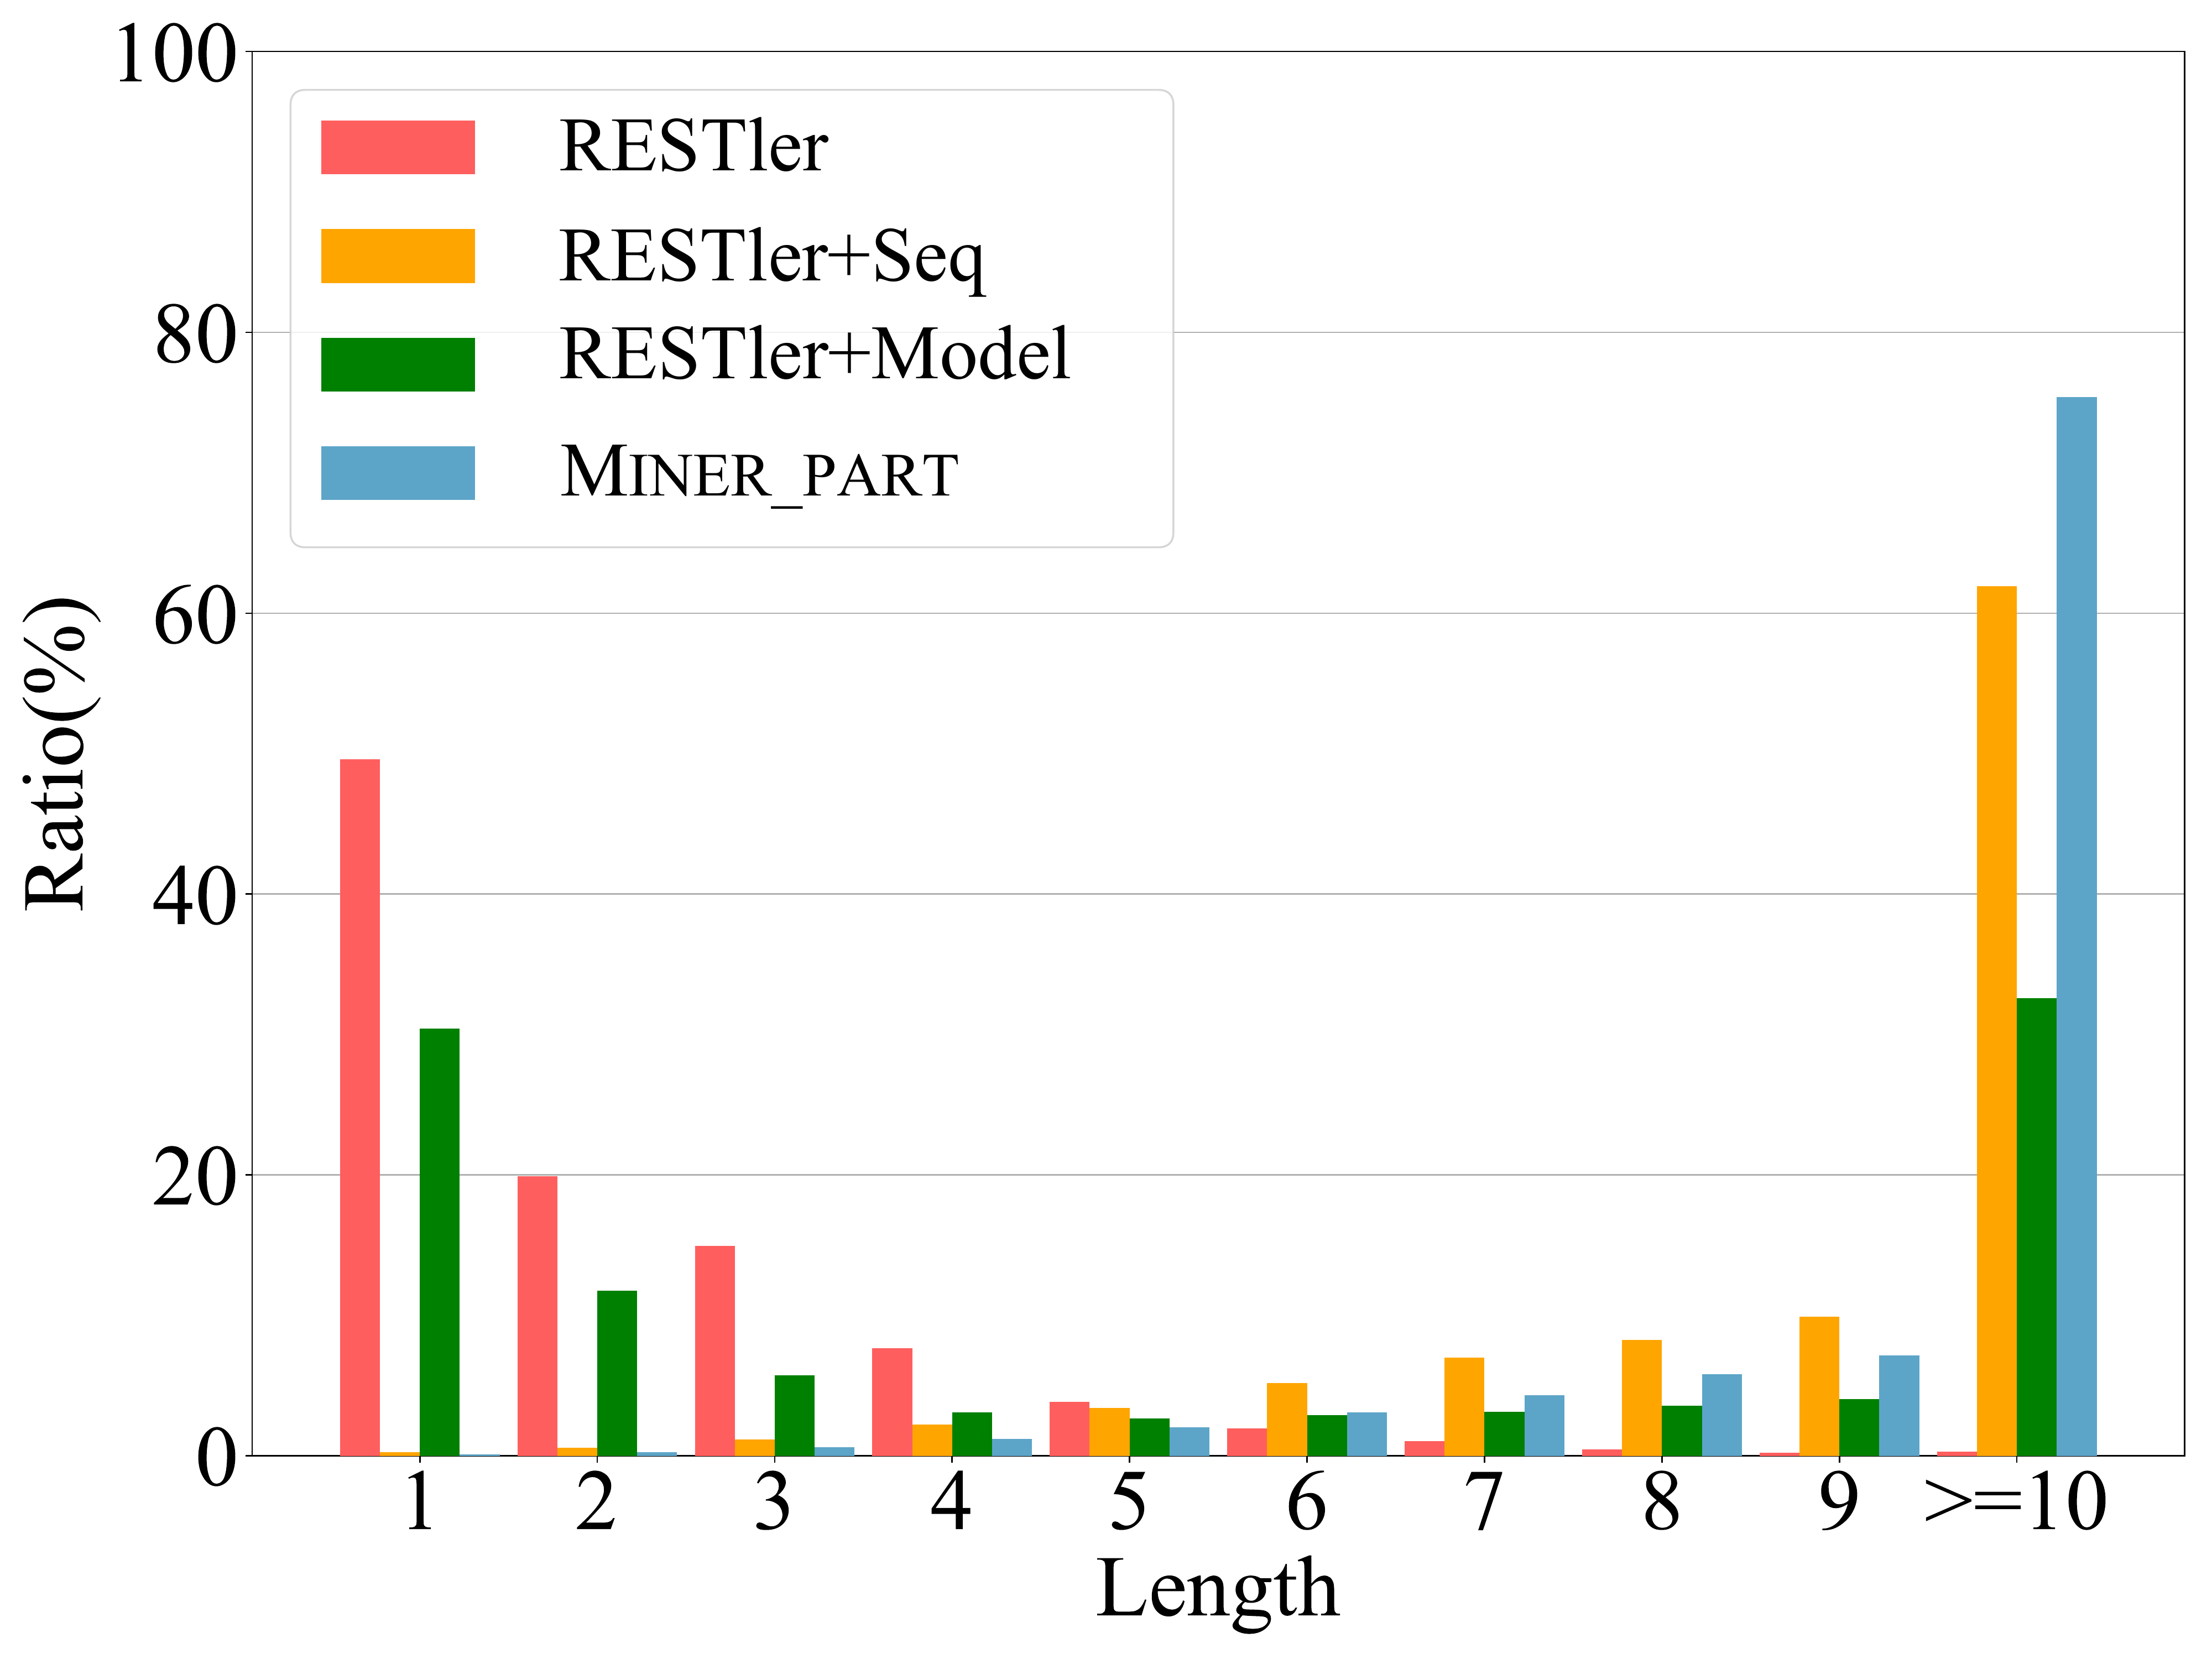}
            \setlength{\abovecaptionskip}{-0.4cm}
            \caption{Wordpress Categories API.}
            %\label{fig:three sin x}
        \end{subfigure}

            \caption{The distribution of  sequence length sent by RESTler, RESTler+Seq, RESTler+Model and \sysnamepart, where RESTler+Seq only implements the \emph{length orientated sequence construction} and RESTler+Model only implements the \emph{attention model-based request generation}.} % to generate \textit{parameter combinations}.} 
            \label{fig:seqlength} 
     \end{minipage}
     
\end{figure*}

$\bullet$
As shown in Fig.~\ref{fig:seqlength}, the \emph{attention model-based request generation} can increase the executions of long request sequences. For instance, RESTler+Model assigns more executions on longer request sequences than RESTler on all 5 targets. \sysnamepart also generates more request sequences with larger lengths compared to RESTler+Seq. The results demonstrate the contribution of the \emph{attention model-based request generation} to sequence extension. By improving the pass rate of requests with our design, a REST API fuzzer can construct valid request sequences with larger length.

$\bullet$
The \emph{length orientated sequence construction} significantly increases the executions of request sequences with large length. For instance, both \sysnamepart and RESTler+Seq assign most executions to the request sequences of length greater than 10, demonstrating our design's effectiveness. 
%. The results demonstrate the effectiveness of our design. 

\section{Coverage Performance Analysis}\label{sec:coverage}

\begin{figure*}[t]
    \setlength{\abovecaptionskip}{0.2cm}
    \setlength{\belowcaptionskip}{-0.3cm}
     \centering
     \begin{subfigure}[b]{0.32\textwidth}    
         \centering
         \includegraphics[width=2.35in,height=1.8in]{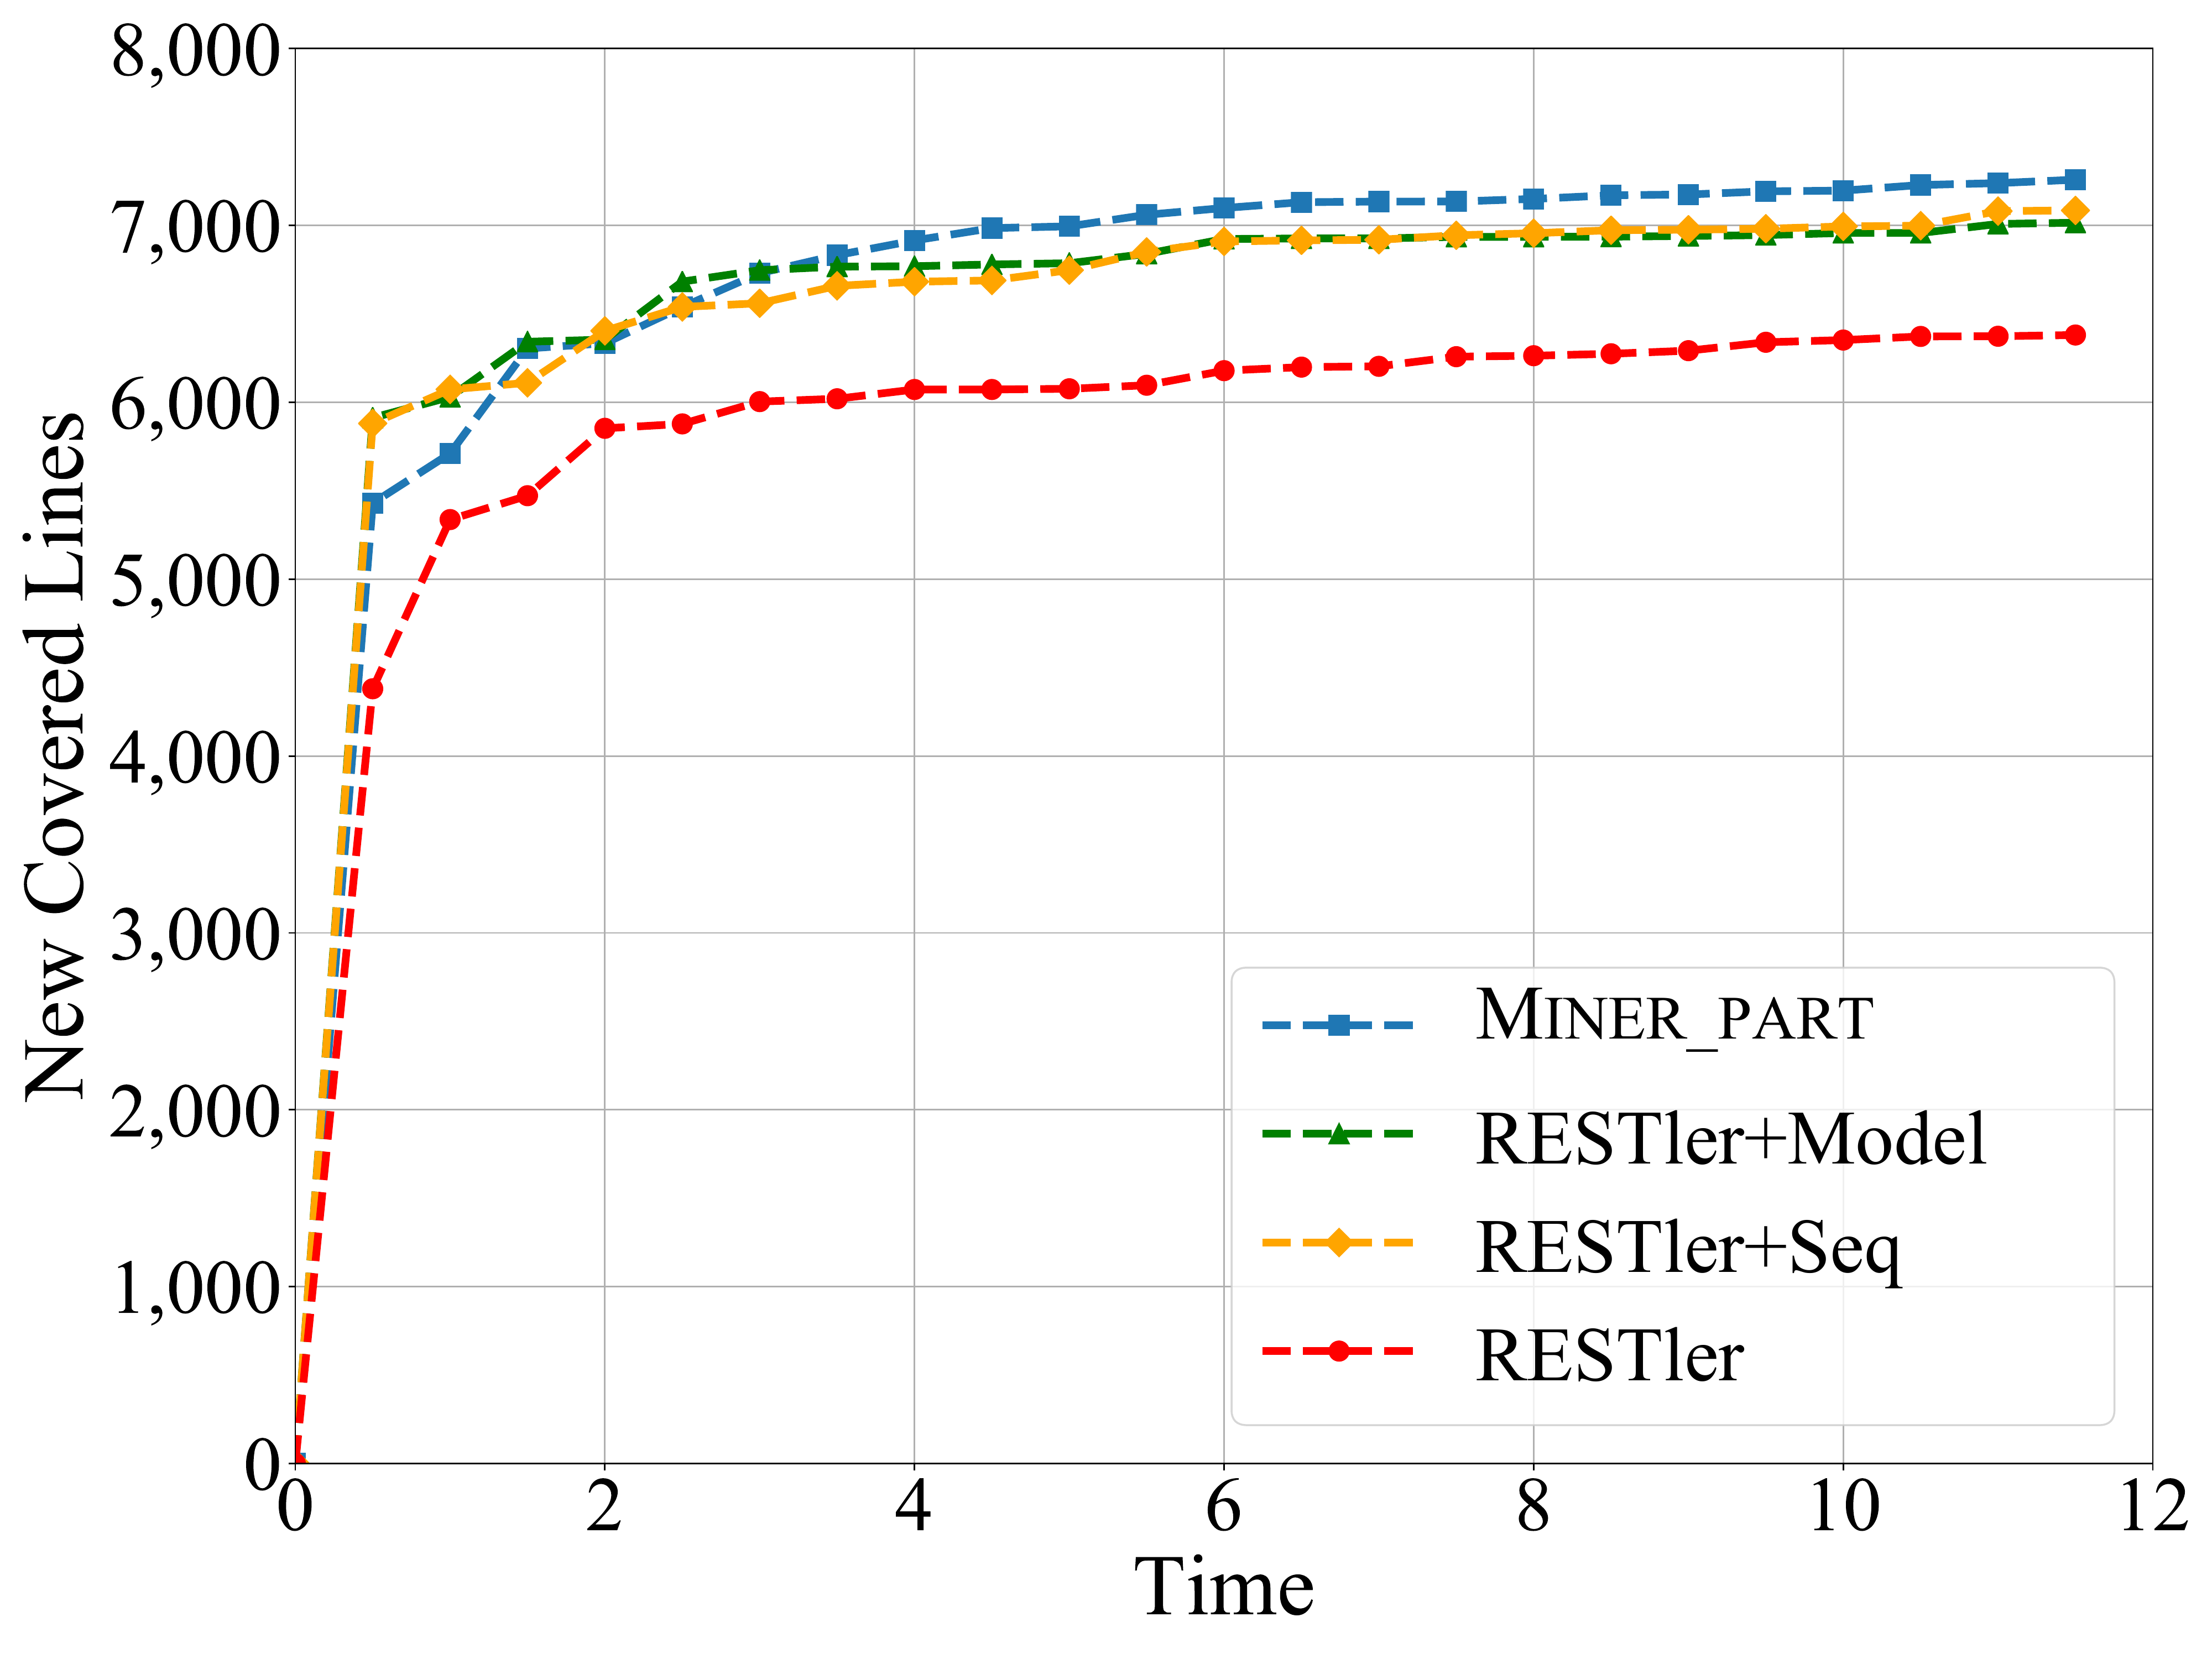}
         \caption{GitLab Projects API.}
         %\label{fig:y equals x}
     \end{subfigure}
     \hfill
     \begin{subfigure}[b]{0.32\textwidth}
         \centering
         \includegraphics[width=2.35in,height=1.8in]{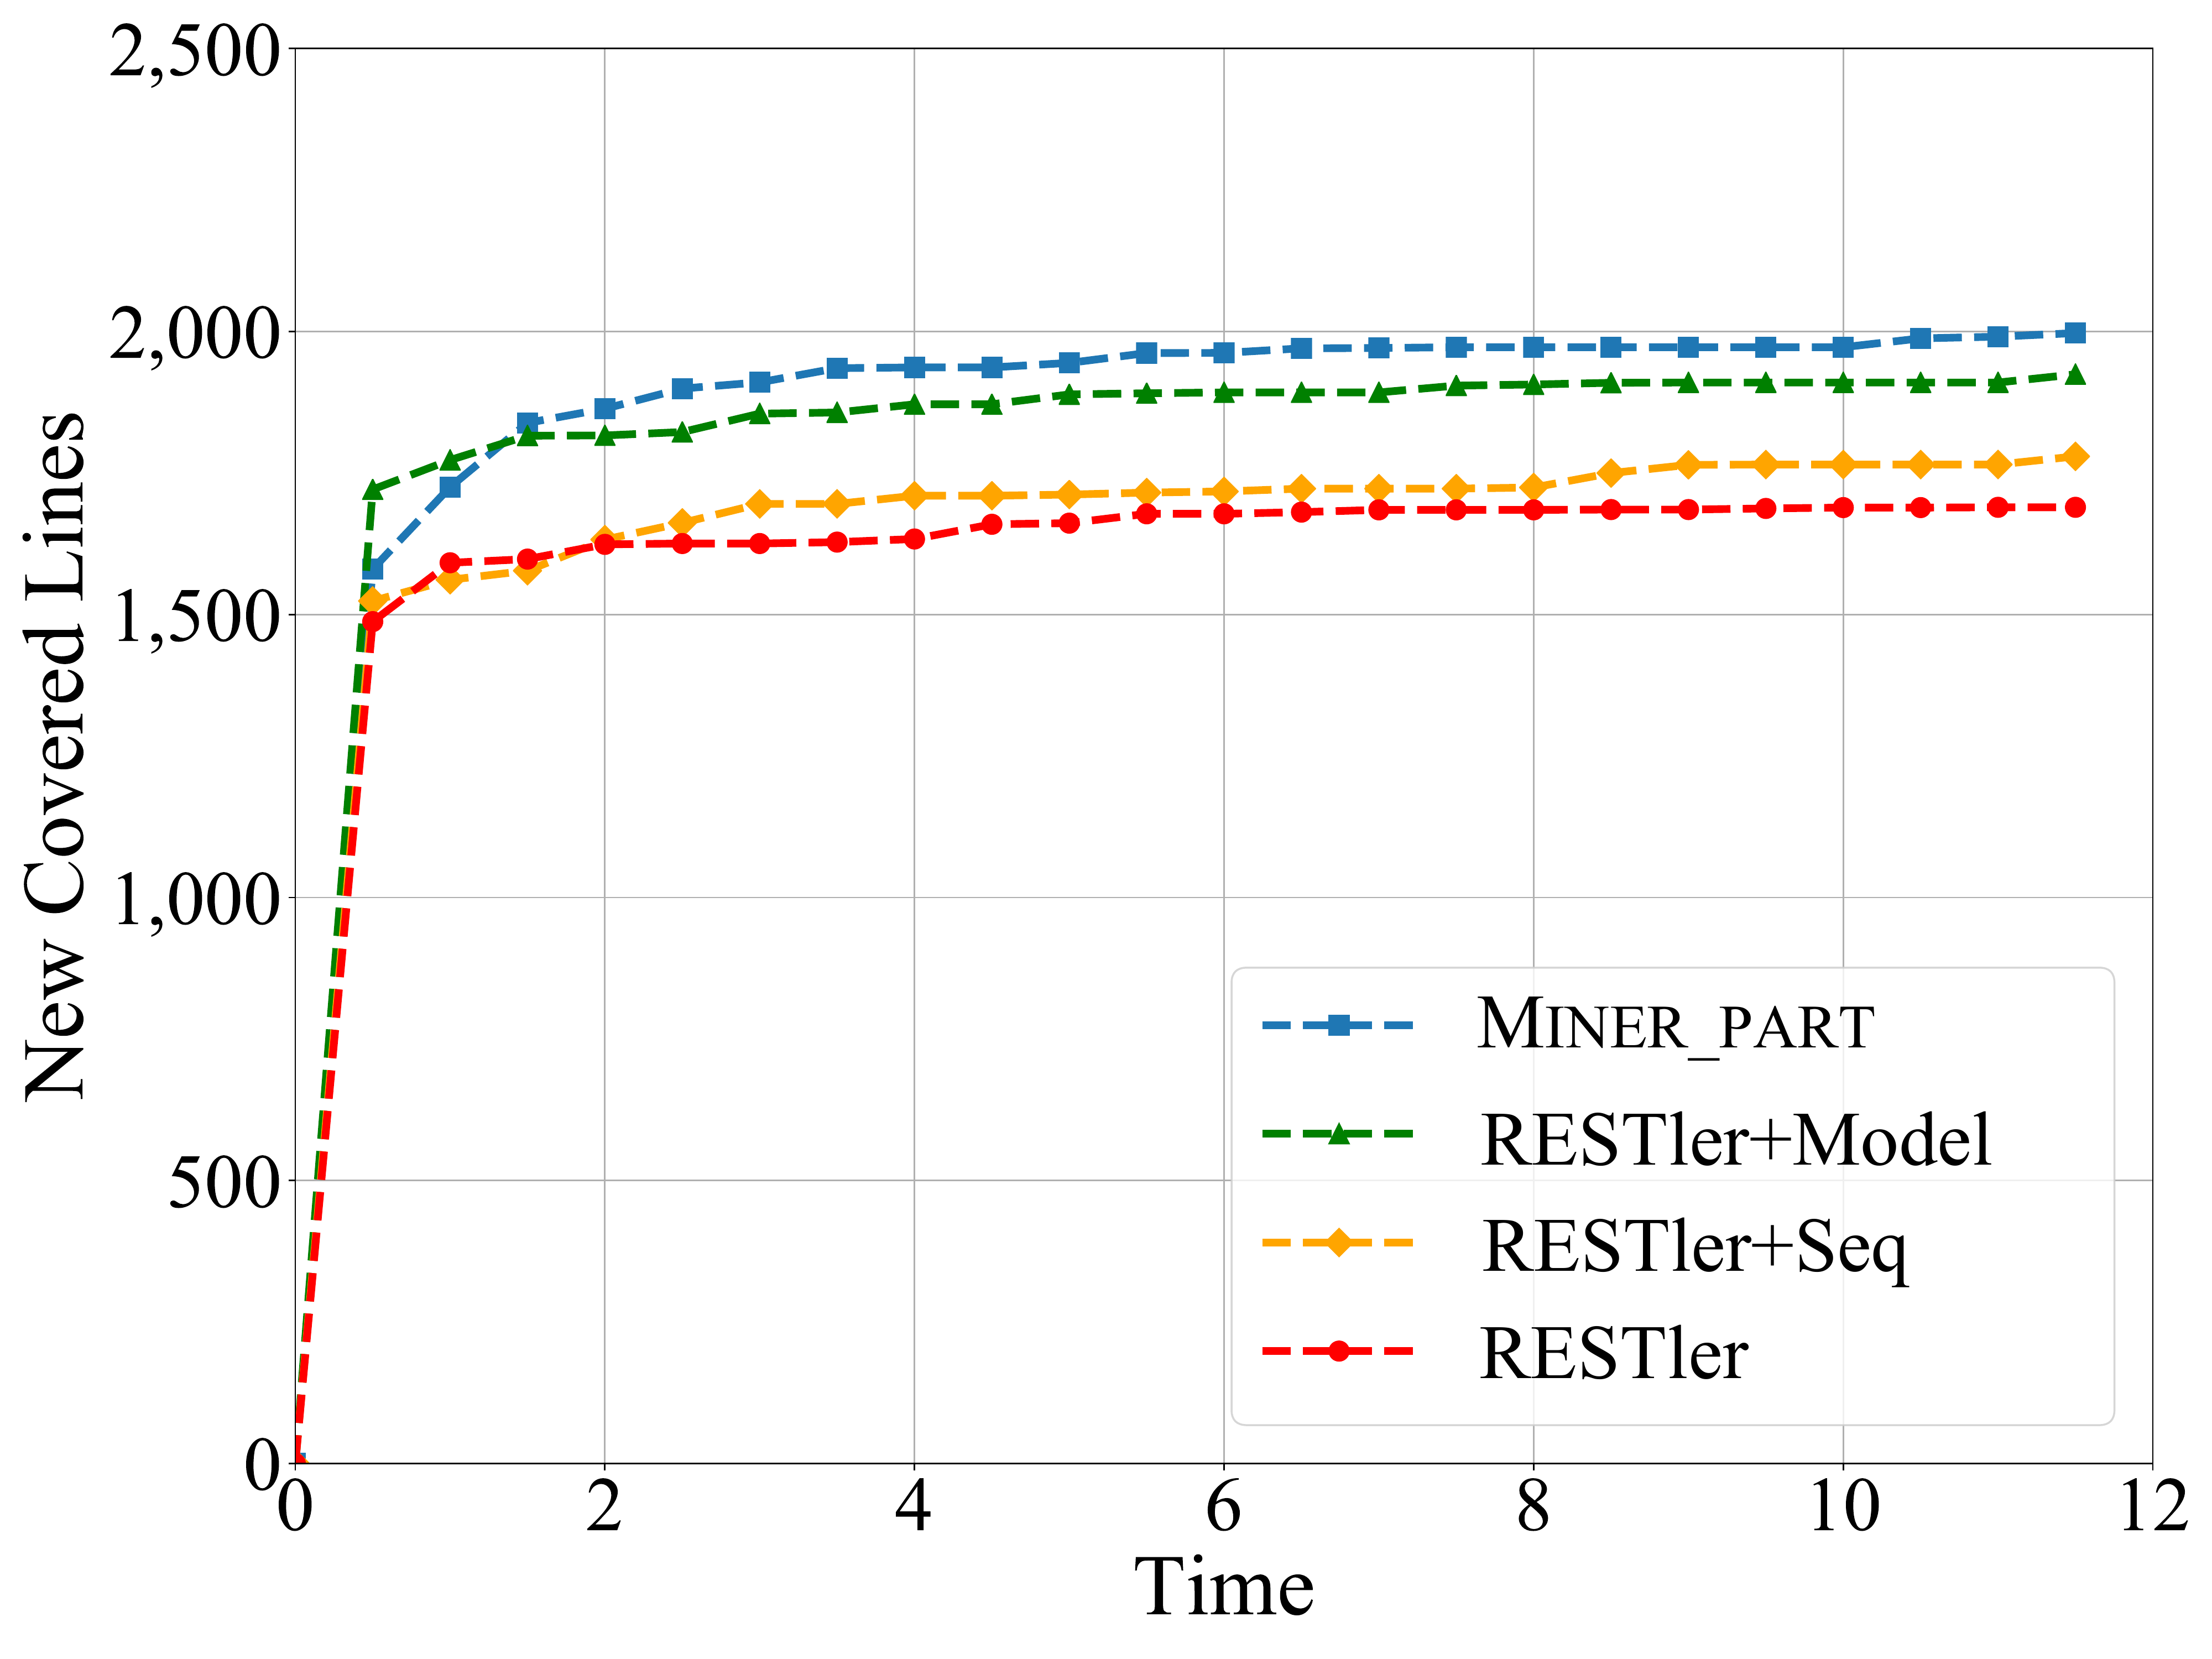}
         \caption{GitLab Groups API.}
         %\label{fig:three sin x}
     \end{subfigure}
     \hfill
     \begin{subfigure}[b]{0.32\textwidth}
         \centering
         \includegraphics[width=2.35in,height=1.8in]{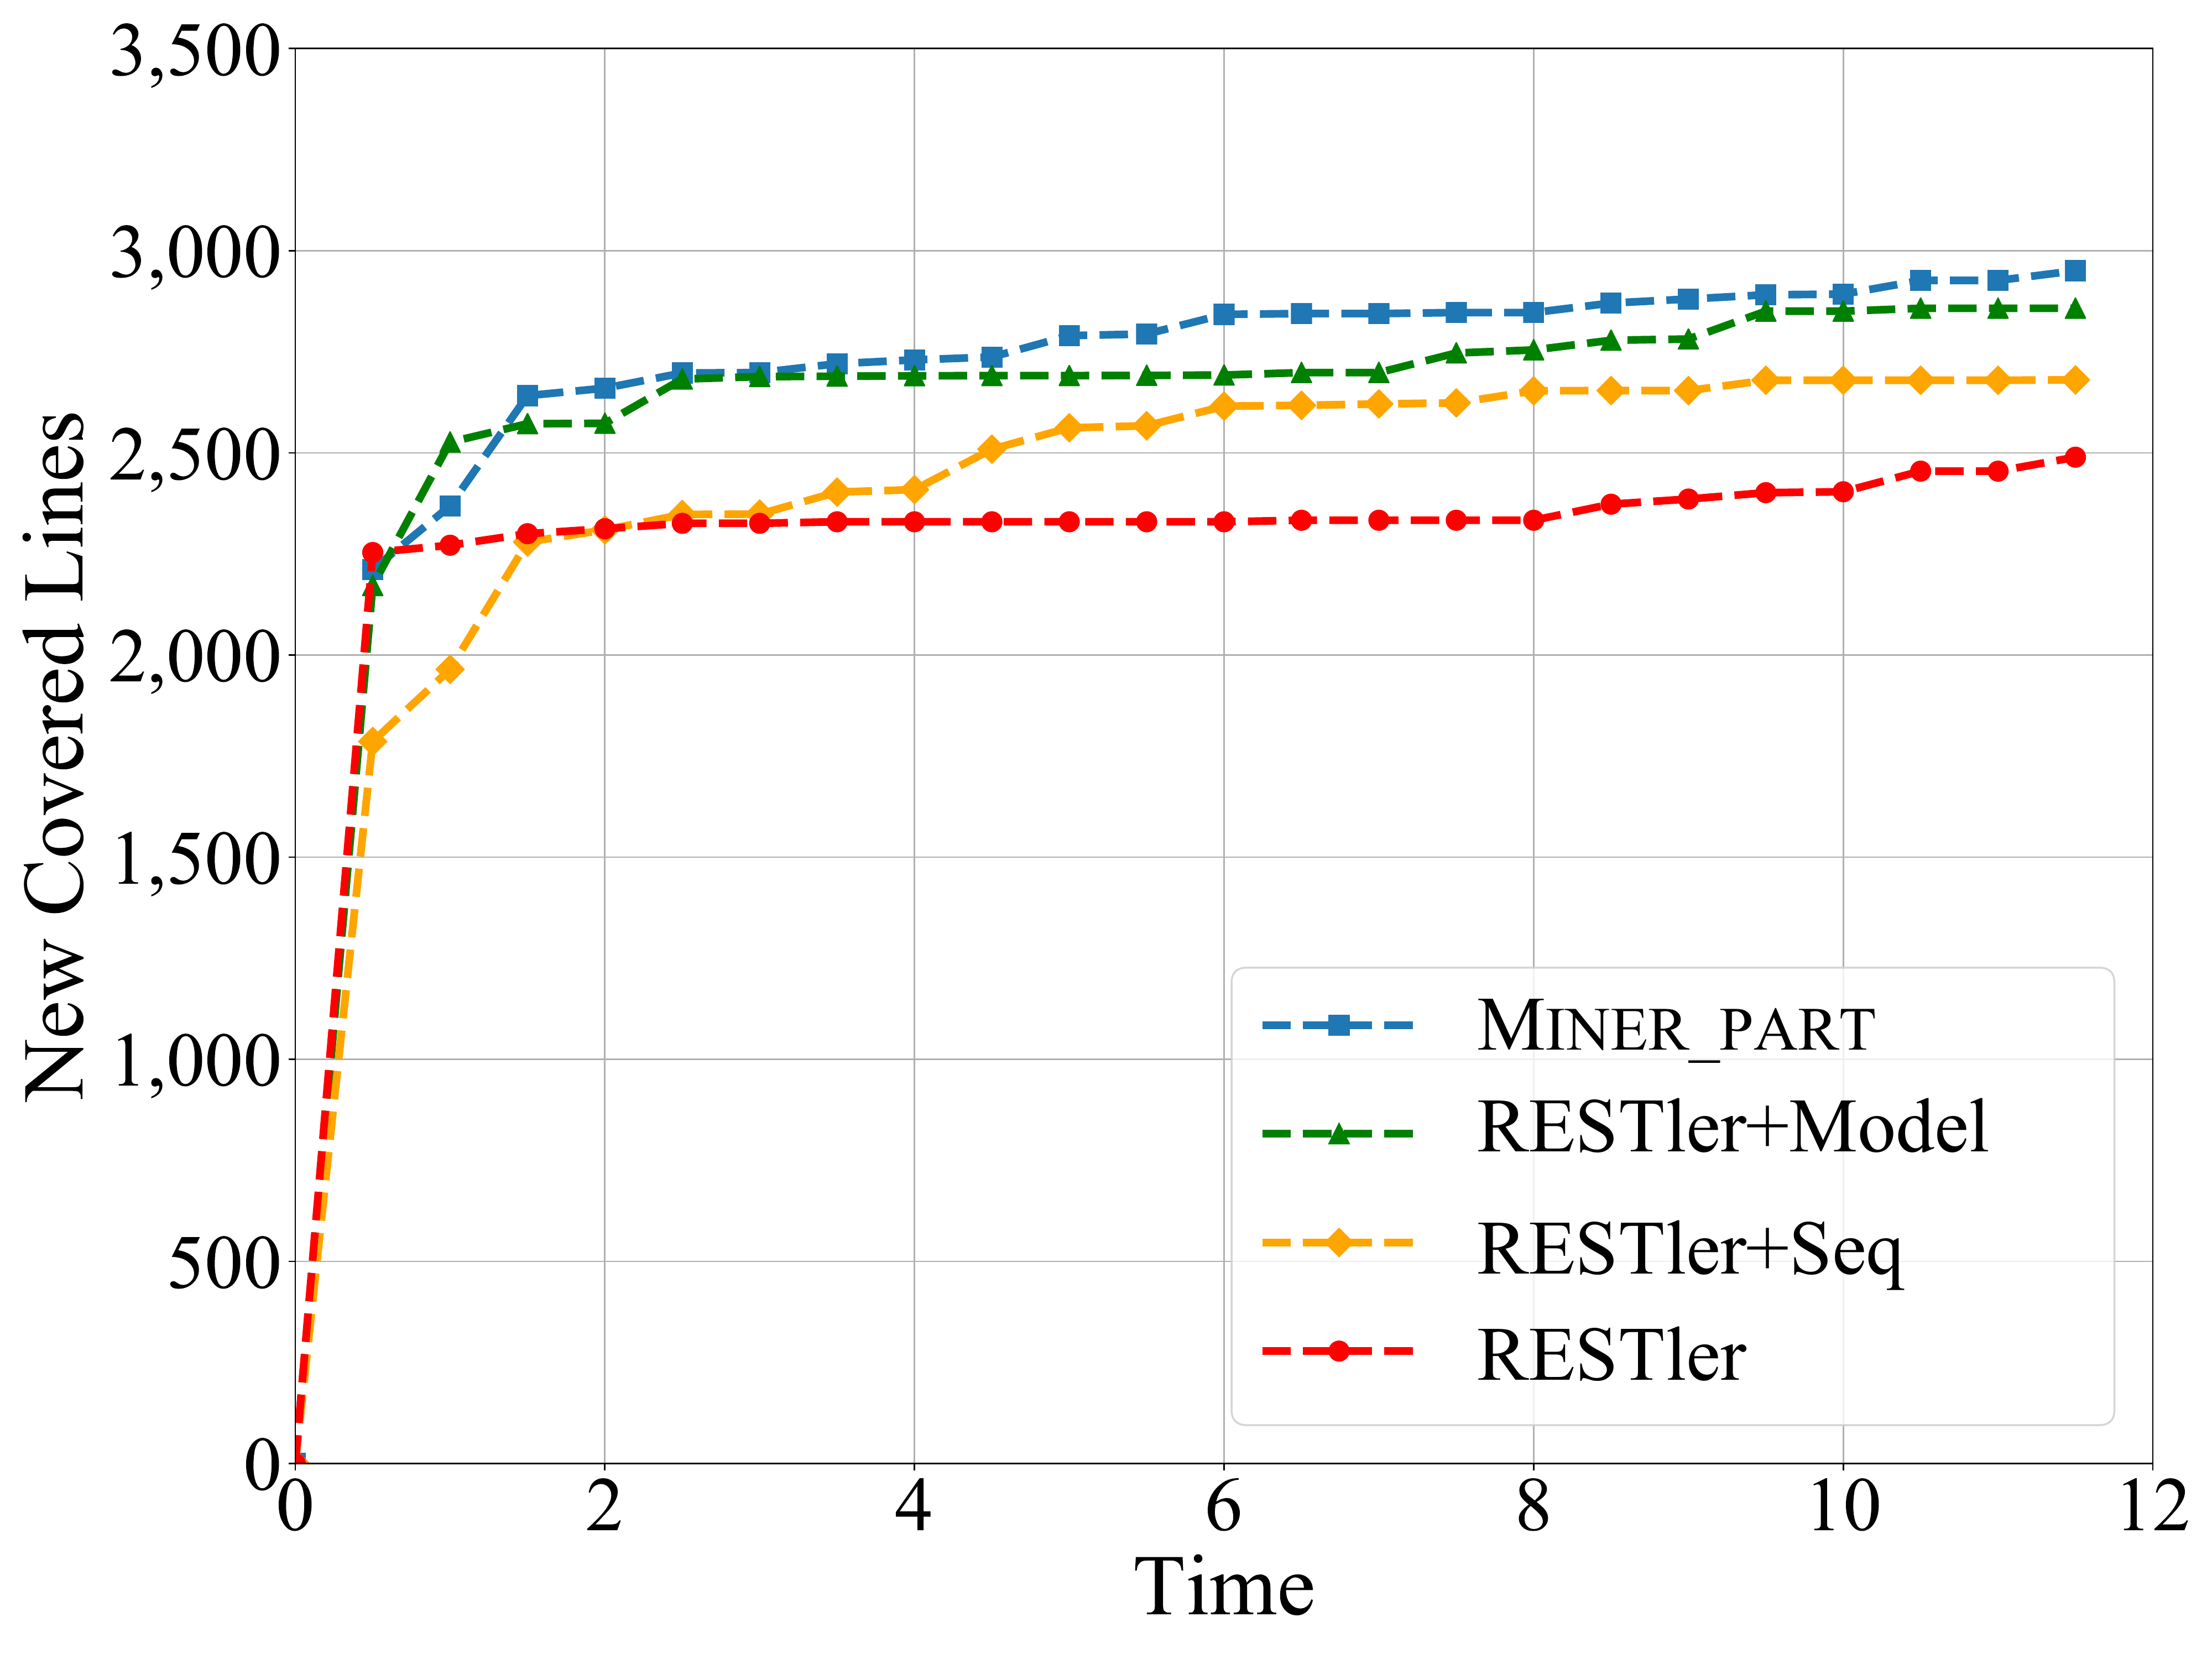}
         \caption{GitLab Issues API.}
         %\label{fig:five over x}
     \end{subfigure}
     \hfill
     \vspace{0.5cm}
     
     \begin{minipage}[!htb]{1\linewidth}
     \centering
     
        \begin{subfigure}[b]{0.32\textwidth}
            \centering
            \includegraphics[width=2.35in,height=1.8in]{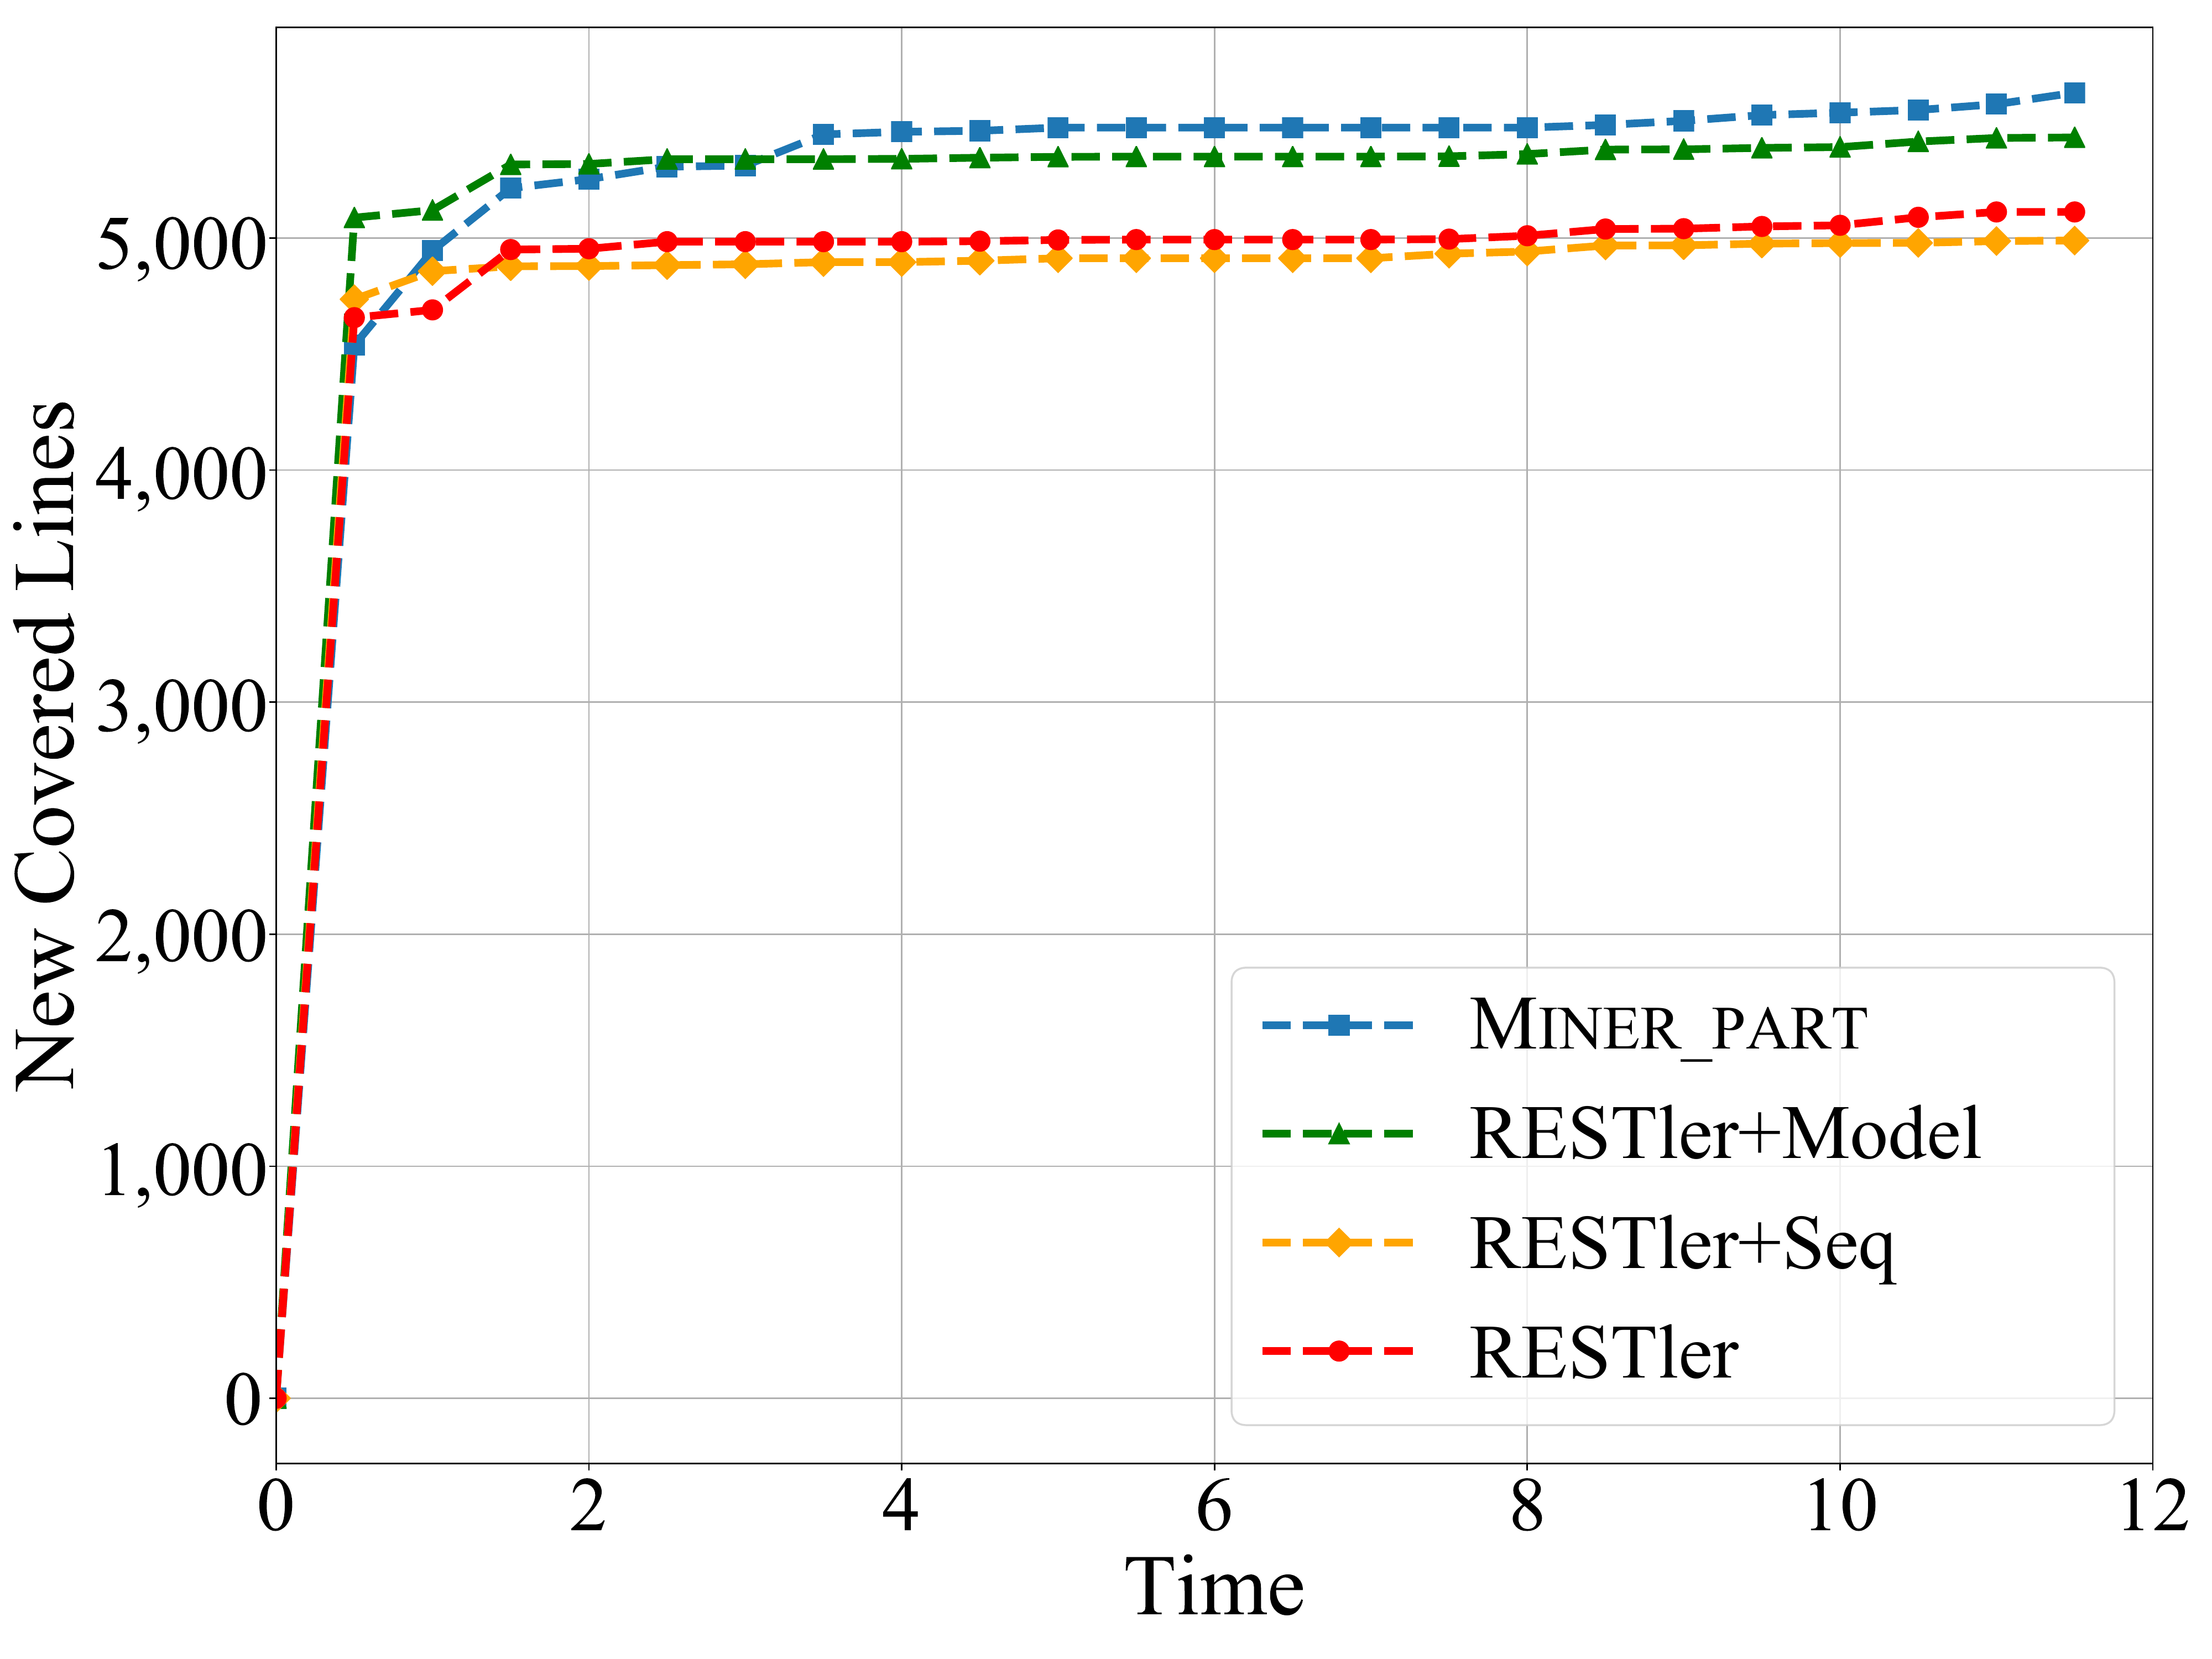}
            \caption{GitLab Commits API.}
            %\label{fig:three sin x}
        \end{subfigure}
        \hspace{4mm}
        \begin{subfigure}[b]{0.32\textwidth}
            \centering
            \includegraphics[width=2.35in,height=1.8in]{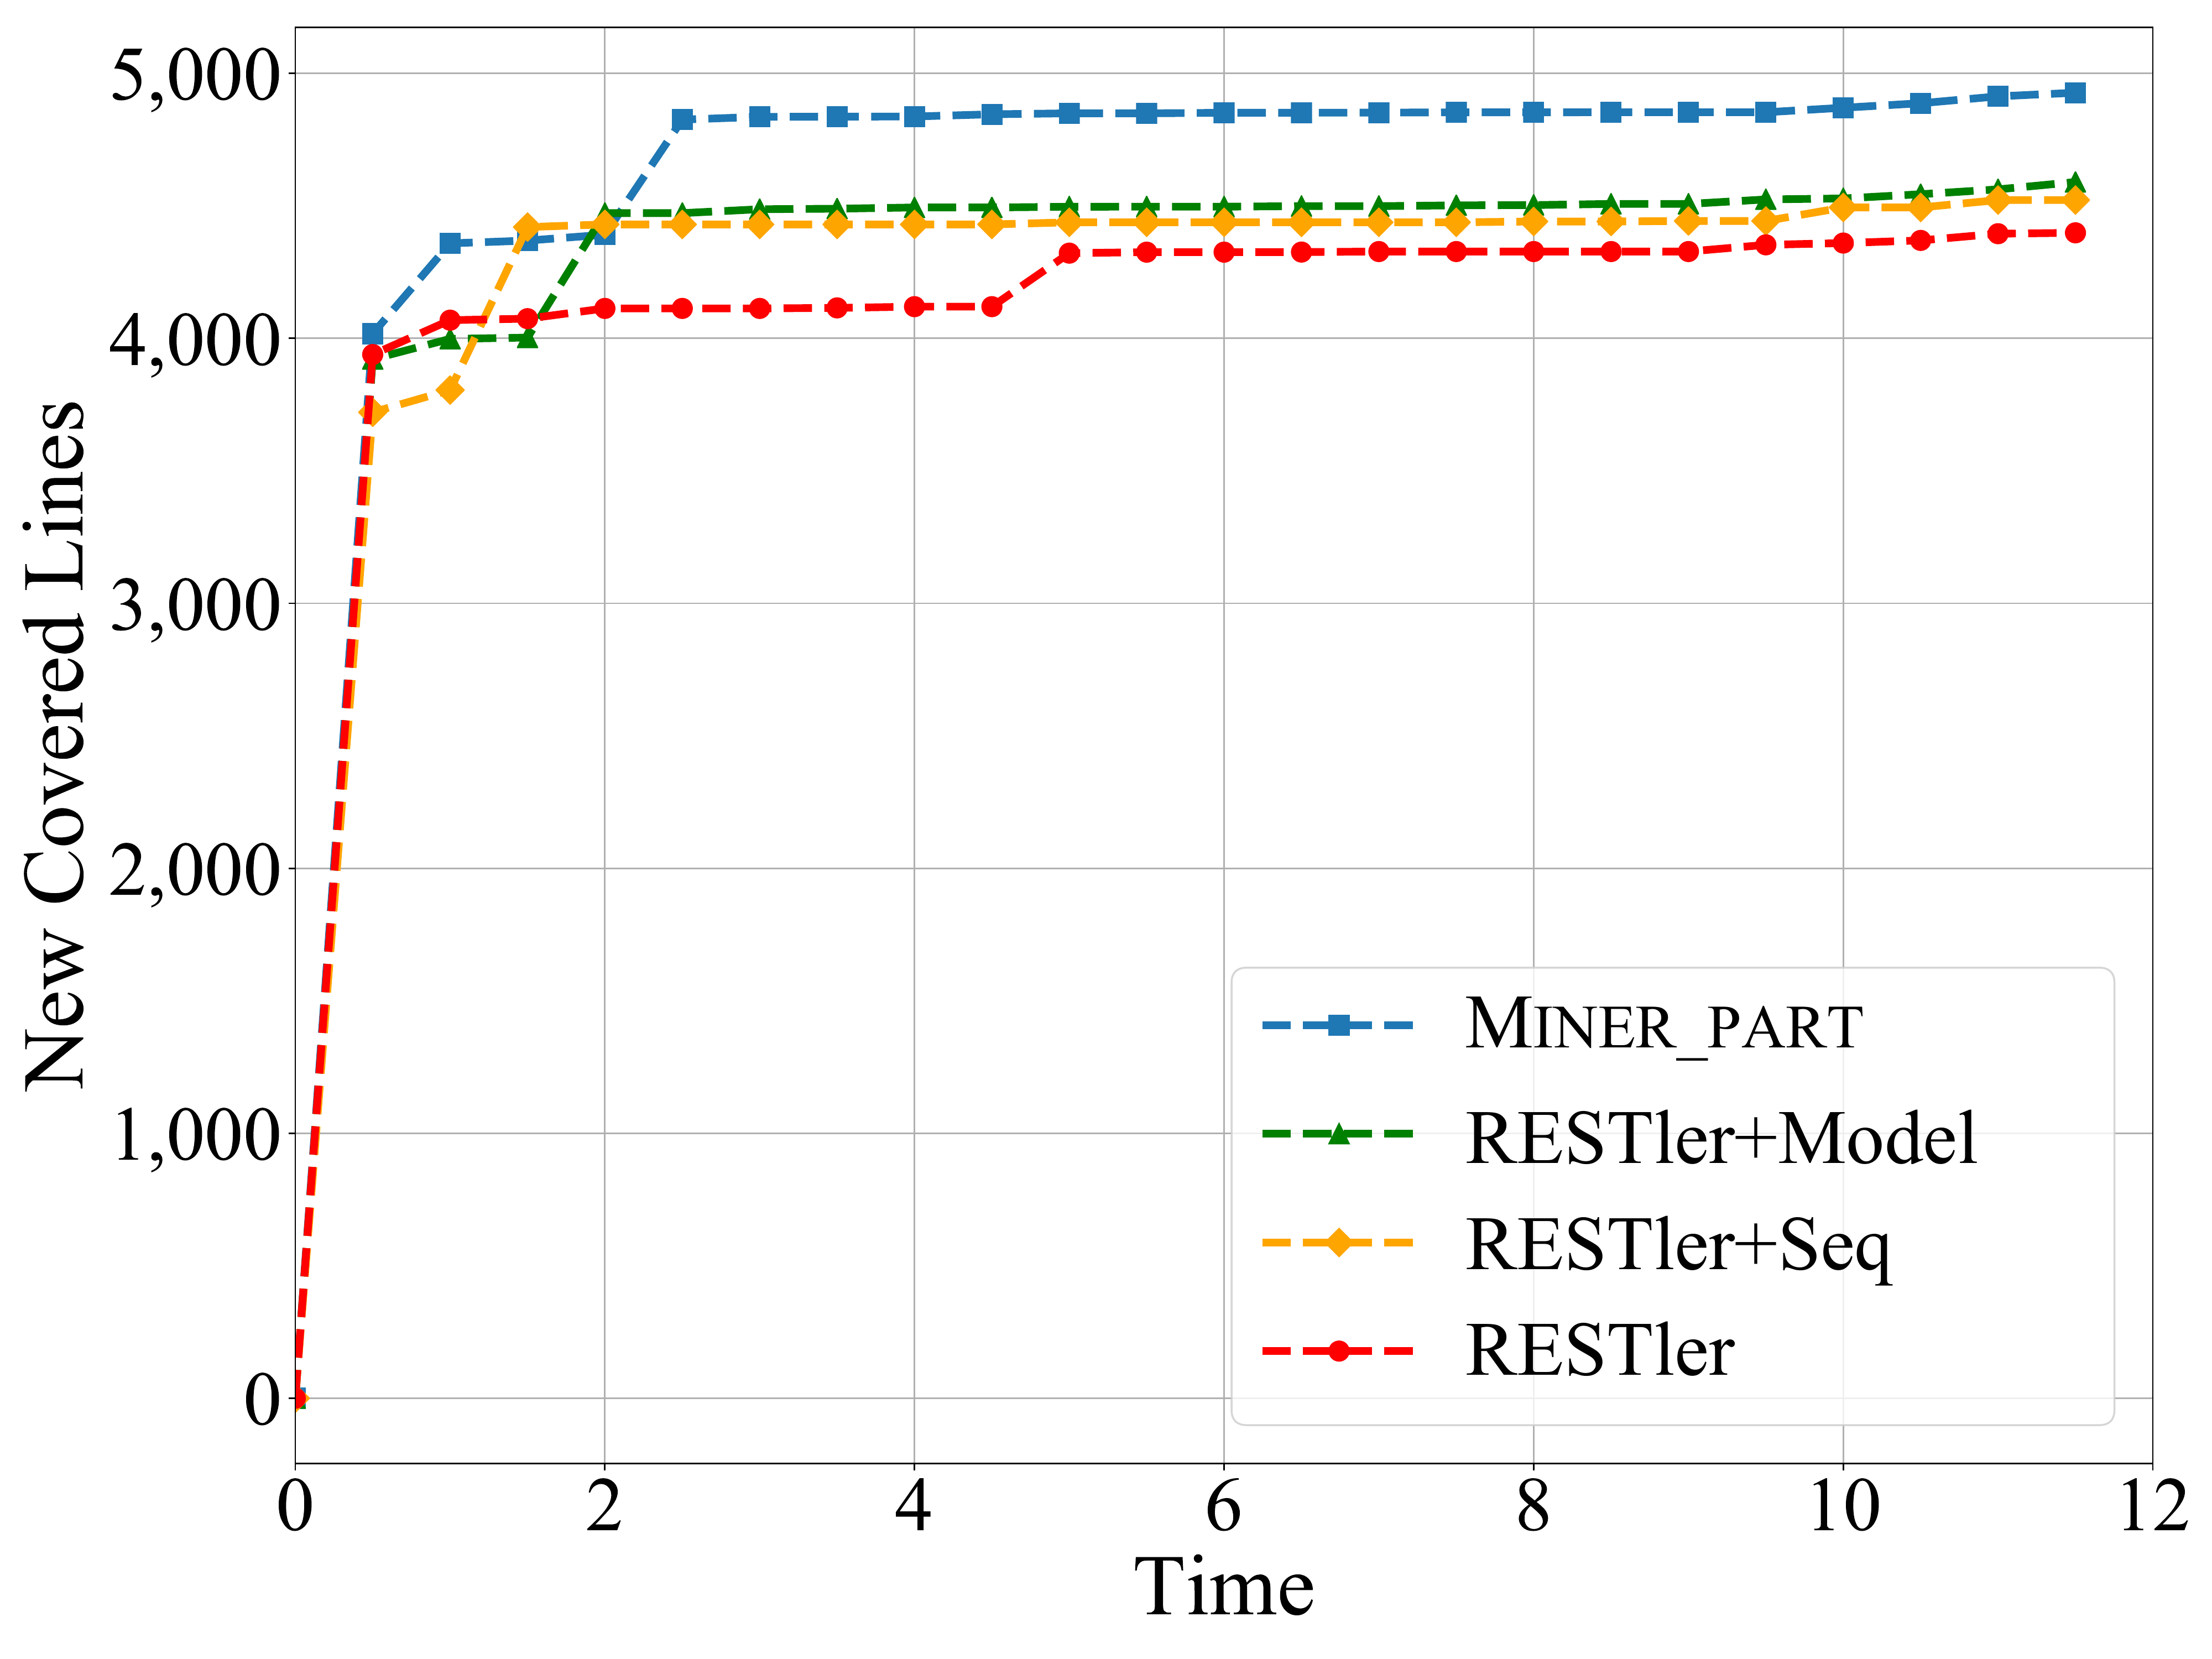}
            \caption{GitLab Branches API.}
            %\label{fig:five over x}
        \end{subfigure}
            \caption{The line coverage growth of  4 fuzzers when fuzzing GitLab through its 5 REST APIs, respectively.}
            \label{fig:coveredlines}
     \end{minipage}
\end{figure*}

In order to evaluate the coverage performance of each fuzzer, 
we hook the source code of GitLab to trace the number of covered code lines triggered by the incoming requests. 
%\JC{Specifically, we leverage a popular ruby gem \texttt{Coverband}\cite{coverband}, which allows easy configuration to collect and report on production code usage, to trace lines of codes executed in GitLab's \texttt{service/lib} and \texttt{service/app} folders.} 
%Specifically, we leverage a popular ruby gem named \emph{Coverband}\cite{coverband} to collect and report the production code usage, which traces the code lines executed in GitLab's \texttt{service/lib} and \texttt{service/app} folders. 
Specifically, we leverage a popular ruby gem named \emph{Coverband}~\cite{coverband} to trace the code lines executed in GitLab's \texttt{service/lib} and \texttt{service/app} folders. 
We also exclude the coverage statistics for irrelevant behaviors like service boot. 
Then, we conduct the line coverage evaluation for RESTler, RESTler+Seq, RESTler+Model, and \sysnamepart, 
each of which lasts for 12 hours. 
Since the \emph{DataDriven Checker} reuses the \textit{<parameter, value> pairs}
collected from the valid requests and triggers the repeated code lines, 
it does not affect line coverage. 
Thus, we omit \sysname in the evaluation. 
%Note that we exclude the coverage statistics for irrelevant behaviors like service boot, 
%and the line coverage is definitely incremental during testing.
%Then, we conduct the evaluations of RESTler, \sysname and \sysnameplus 
%to measure their coverage performance on Gitlab, 
The line coverage growth of each fuzzer is shown in Fig.~\ref{fig:coveredlines}, 
from which we have the following observations.

$\bullet$
The results demonstrate the contribution of our designs to line coverage. 
Both the \emph{attention model-based request generation} and \emph{length orientated sequence construction} can improve the line coverage of a REST API fuzzer. For instance, the line coverage of RESTler+Model is better than RESTler on all 5 evaluations. RESTler+Seq also performs significantly better than RESTler on line coverage when fuzzing GitLab Issues API and GitLab Projects API. On the other hand, the line coverage of RESTler+Model is better than RESTler+Seq on most evaluations, which implies that a valid sequence with diverse requests triggers more complicated behaviors of a cloud service than a long sequence with easy-to-construct requests. %as analyzed in Section \ref{sec:stepwise}.   

\begin{table*}[t]
  \setlength{\abovecaptionskip}{0.1cm}
\centering
\caption{The average computational overhead of the attention model and 
the pass rate of requests sent by \sysnamepart  
when the iteration duration of the \texttt{Training Module} is 1 hour, 2 hours and 3 hours, respectively.} \label{table:passrate}
\begin{tabular}{ccc|cc|cc} 
\toprule
\multirow{2}{*}{Target} & \multicolumn{2}{c|}{1 Hour} & \multicolumn{2}{c|}{2 Hours} & \multicolumn{2}{c}{3 Hours}  \\ 
\cline{2-7}
               & Overhead  & Pass Rate  & Overhead    & Pass Rate  & ~Overhead     & Pass Rate     \\ 
%\hline
\toprule
GitLab Projects API    & {346.20s}  &   {92.78\%}        &  {380.80s}        &  {91.54\%}            &  {989.30s}         &    {89.55\%}            \\ 
\hline
GitLab Groups API     &  318.90s     & 93.49\%            & 386.90s & 92.80\%                &   1,002.67s   & 91.92\%                  \\ 
\hline
GitLab Issues API      & {463.40s}      & {90.90\%}            & {498.67s}          & {90.67\%}               & {1,001.60s}       &{90.23\%}   \\
\hline
GitLab Commits API     & {29.00s}      & {86.66\%}            & {35.60s}          & {84.45\%}               & {82.33s}       &{82.56\%}   \\
\hline
GitLab Branches API      & {{16.70s}}      & {{90.72\%}}            & {{34.40s}}          & {{87.83\%}}               & {{43.33s}}       &{{86.78\%}}   \\
\bottomrule
\end{tabular}
\end{table*}

$\bullet$
\sysnamepart performs the best on line coverage on all 5 evaluations. For instance, \sysnamepart covers the most code lines at the end of each evaluation.  The line coverage triggered by \sysnamepart grows rapidly on GitLab Groups API and GitLab Branches API. The results demonstrate that our data-driven designs can be combined to improve the line coverage performance of a REST API fuzzer.

%\section{Overhead and Pass Rate Analysis with Different \texttt{Training Module}}\label{sec:overheadandpassrate}

\section{Iteration Schedule of the \texttt{Training Module}}\label{sec:overheadandpassrate}

To evaluate the impact of different iteration schedules of the \texttt{Training Module} on fuzzing performance, we measure the computational overhead and pass rate for \sysnamepart when using 1 hour, 2 hours and 3 hours as the iteration duration of the \texttt{Training Module}, respectively. Each evaluation lasts for 12 hours. Thus, the invocation times of the \texttt{Training Module} are 12, 6 and 4 when using the above iteration durations, respectively. For each evaluation, we 1) calculate the average computational overhead in each invocation of the \texttt{Training Module} to train the attention model and generate the \textit{parameter combinations}, and 2) calculate the pass rate of requests. The results are shown in Table~\ref{table:passrate}, from which we have the following conclusions. Note that due to the different number of request templates and the different number of parameters in each request template, the number of the collected \textit{<parameter, value> pairs} (i.e., the training data for the attention model) is different when using \sysnamepart to fuzz GitLab through different REST APIs. Thus, the average computational overhead to train the attention model and generate \textit{parameter combinations} can be different when fuzzing GitLab through different REST APIs.

$\bullet$
The average computational overhead to train the attention model and generate \emph{parameter combinations} increases when using a larger iteration duration of the \texttt{Training Module}. For instance, as shown in Table~\ref{table:passrate}, the average computational overhead of the \texttt{Training Module} increases 185.76\% when using 3 hours as the iteration duration to fuzz GitLab Projects API compared to 1 hour. The average computational overhead  increases 100.85\% when using 3 hours as the iteration duration to fuzz GitLab Issues API compared to 2 hours. We analyze the reasons for the results as follows. When the iteration duration of the \texttt{Training Module} increases, the training data collected  in the \texttt{Collection Module}  increases correspondingly. Thus, the training set of the attention model increases, which requires more time to train the model. Note that although the average computational overhead increases when the iteration duration increases, the invocation times of the \texttt{Training Module} decrease. Therefore, there is no distinct difference in the total computational overhead under different iteration durations.

%\vspace{1cm}
\begin{figure}
    \setlength{\abovecaptionskip}{0.01cm}
    \setlength{\belowcaptionskip}{0.1cm}
        \centering
        \begin{subfigure}[b]{0.5\textwidth}    
            \centering
            \includegraphics[width=3.2in,height=1.65in]{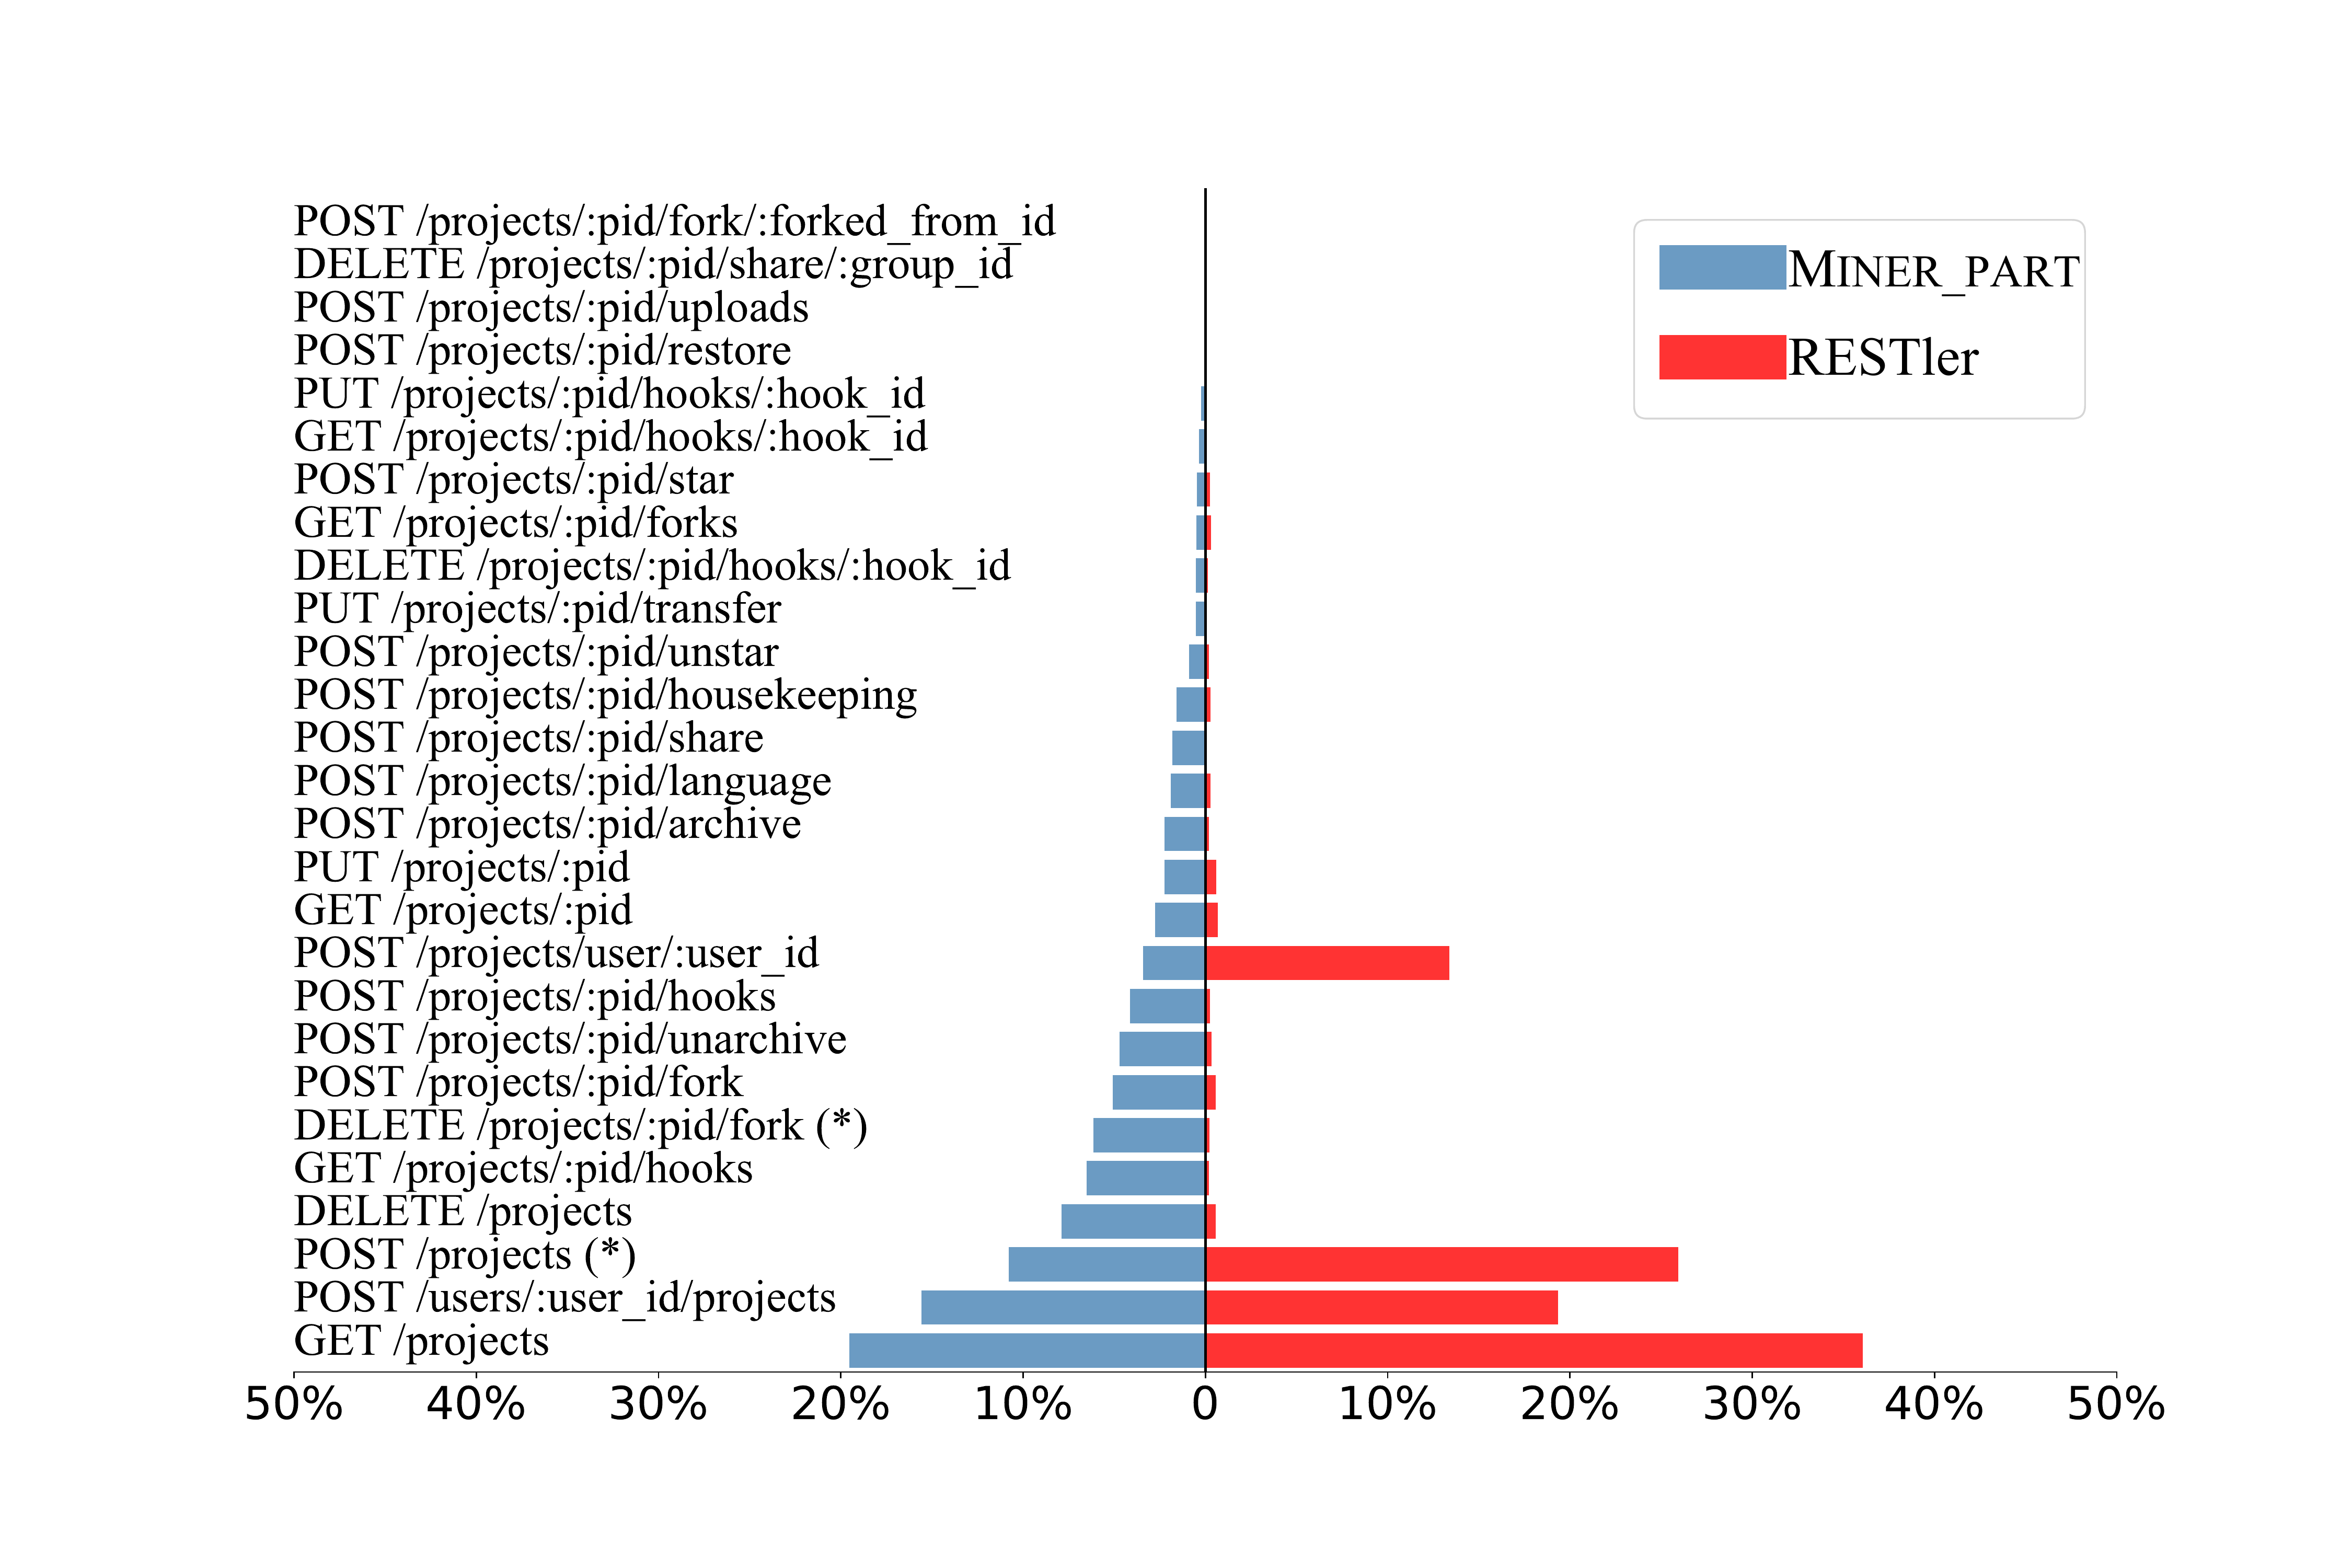}
            \caption{GitLab Projects API.}
            %\label{fig:y equals x}
        \end{subfigure}
        \hfill
        \begin{subfigure}[b]{0.5\textwidth}
            \centering
            \includegraphics[width=3.2in,height=1.65in]{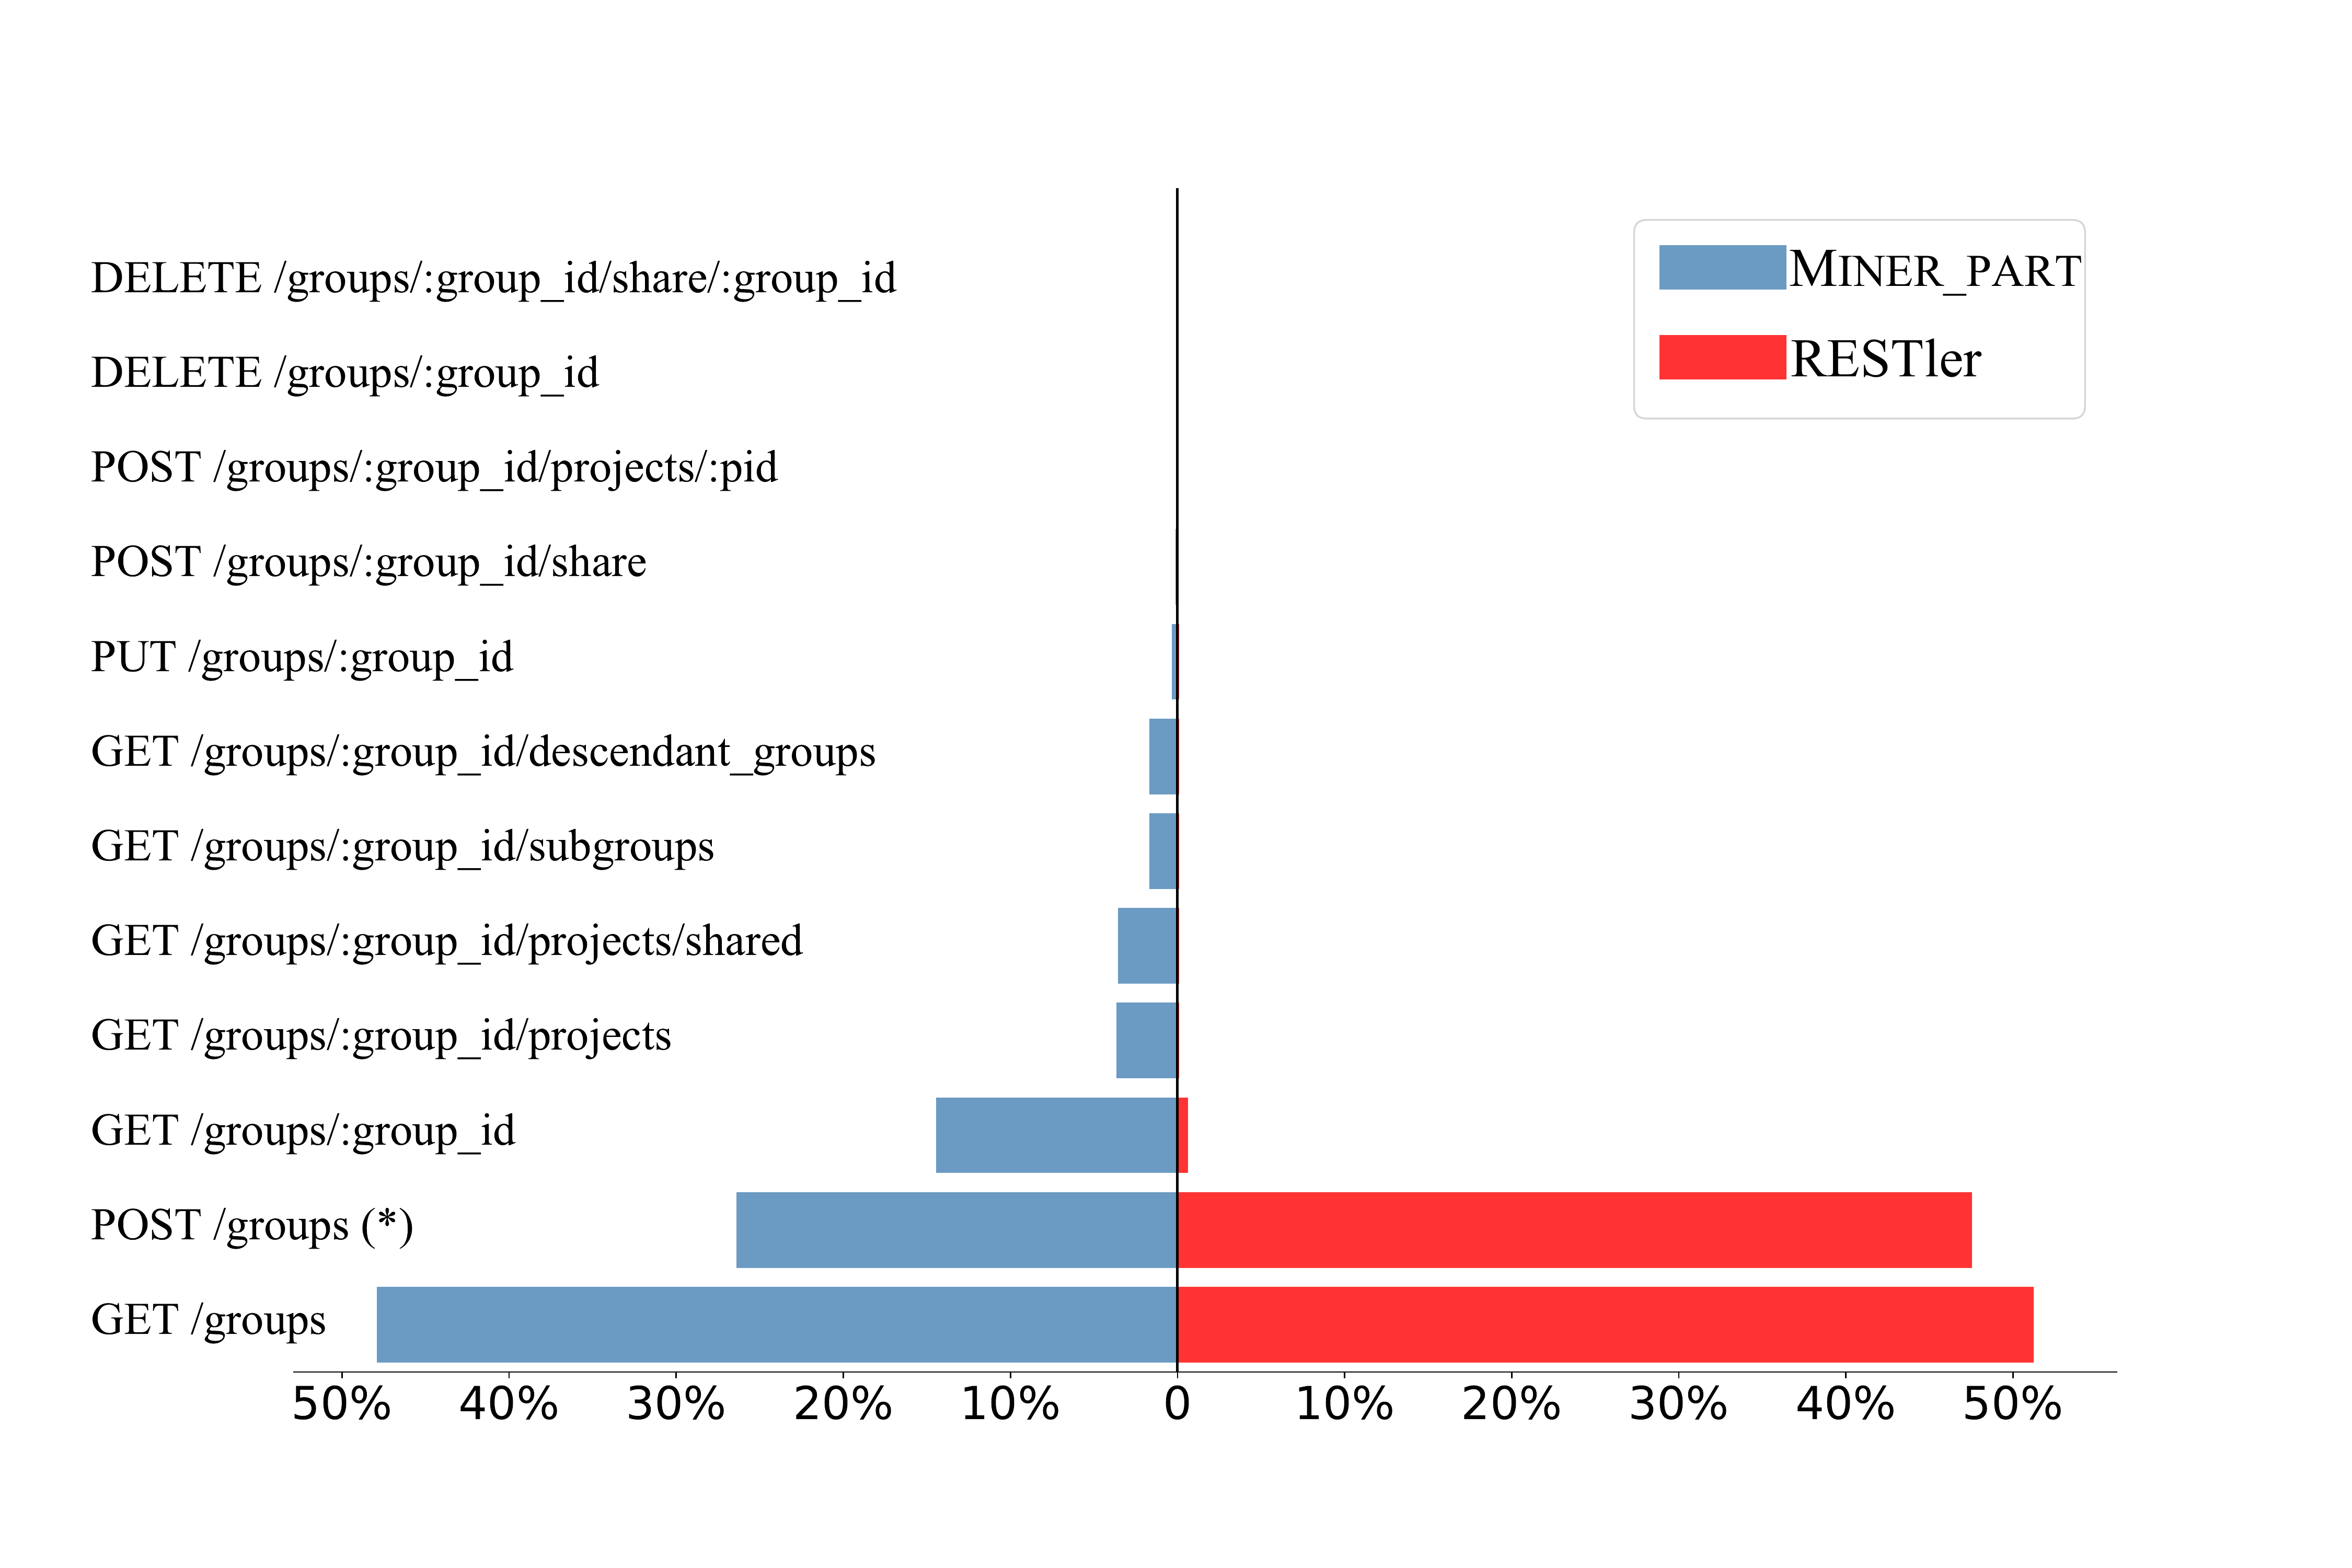}
            \caption{GitLab Groups API.}
            %\label{fig:three sin x}
        \end{subfigure}
        \hfill
        \begin{subfigure}[b]{0.5\textwidth}
            \centering
            \includegraphics[width=3.2in,height=1.65in]{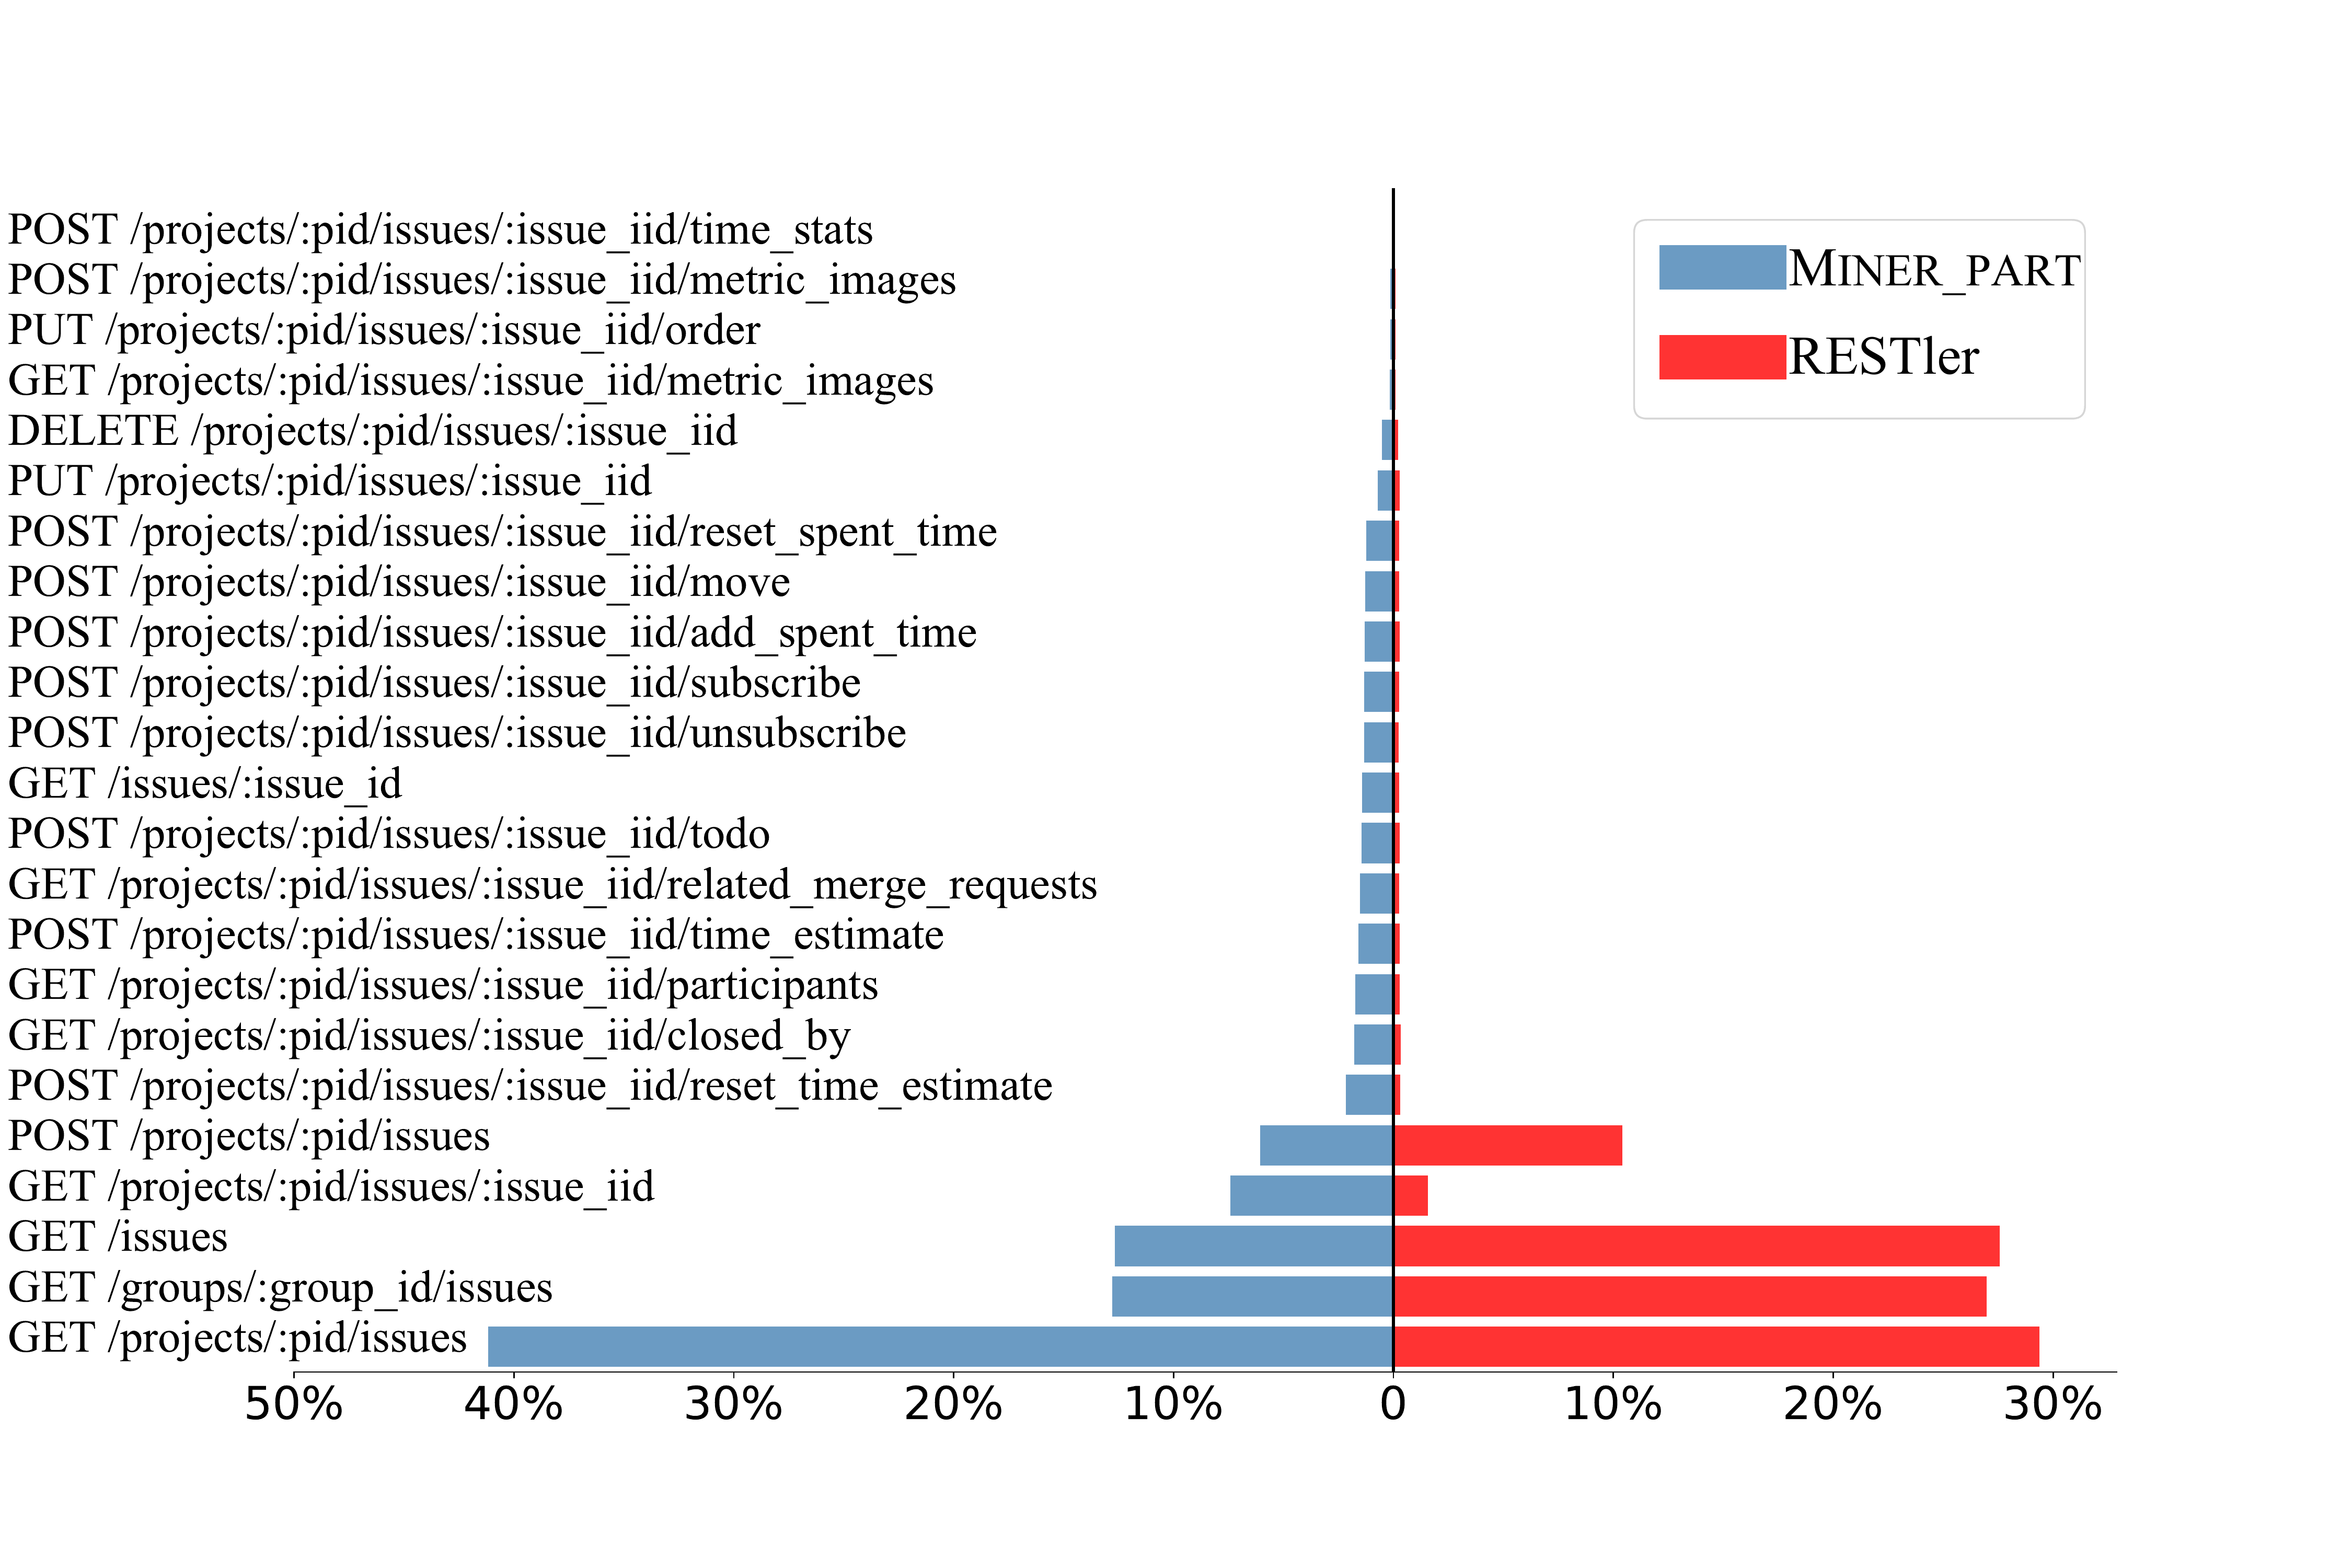}
            \caption{GitLab Issues API.}
            %\label{fig:five over x}
        \end{subfigure}
           \caption{The distribution of executions of different request templates sent by RESTler and \sysnamepart when fuzzing GitLab via its REST APIs, where the request template with $(*)$ means that it has multiple versions in order to provide different target object ids.} 
           \label{fig:executions}     
   \end{figure}

$\bullet$
We can learn from Table~\ref{table:passrate} that the pass rate is close when using different iteration durations. 
For instance, 
the pass rate of \sysnamepart slightly decreases when using a longer iteration duration to invoke the \texttt{Training Module}. 
The pass rate of \sysnamepart is around 90.50\% when using  different iteration durations to fuzz GitLab Issues API. 
We infer the reasons as follows. 
The slight difference in pass rate is caused by the request generation in the first period, 
in which \sysnamepart does not have the \textit{parameter combinations} generated by the attention model and 
uses the traditional generation method to generate requests with a low pass rate. 
Thus, the longer the iteration duration is, the more times \sysnamepart generates requests with a low pass rate in the first period. 
After the first time invoking the \texttt{Training Module} 
and obtaining \textit{parameter combinations}, 
\sysnamepart improves the generation quality of requests and significantly increases the pass rate. %is up to more than 90\%. 
As a result, when using 3 hours as the iteration duration compared to 1 and 2 hours, 
\sysnamepart generates more requests with the traditional generation method, which results in a slightly lower pass rate.

\section{Execution Distribution of Requests}\label{sec:distributionrequest}

In this subsection, we conduct the analysis to 
count the executions of each template of requests sent by RESTler and \sysnamepart. 
Each evaluation lasts for 12 hours, and 
the distribution of the executions of different request templates 
is shown in Fig.~\ref{fig:executions}, 
from which we have the following conclusion. 
{\sysnamepart assigns more executions to diverse request templates than RESTler.}  
For instance, as shown in Fig.~\ref{fig:executions}, 
\sysnamepart assigns most executions to 16 templates of requests when fuzzing GitLab Projects API. 
On the contrary, RESTler mainly tests GitLab with 4 request templates. 
When fuzzing GitLab Groups API, 
\sysnamepart  assigns significantly more executions to 5 extra request templates compared to RESTler. 
%Therefore, \sysname can 
\iffalse
Since \sysnamepart assigns more executions to different templates of requests, 
\sysnamepart triggers more kinds of behaviors of a target cloud service and 
explores diverse errors by triggering these behaviors  
compared to RESTler. 
\fi
Therefore, based on more different request templates, 
\sysnamepart can  generate more diverse requests with different parameter values  compared to RESTler. 
Then, \sysnamepart triggers more kinds of behaviors of a target cloud service with these requests, 
and explores more unique errors by triggering these behaviors. %compared to RESTler. 
Thus, the aforementioned conclusion can serve as one of the reasons 
that \sysnamepart performs better than RESTler on line coverage and error discovery.

\end{appendix}
